# Supplementary material for: Asynchronous Training of Word Embeddings for Large Text Corpora
Source: arXiv:1812.03825 source file (2018-12-07)
Supplement: Supplementary file 1 [file appendix.tex]

\newpage

\appendix
\section{Theoretical Analysis}
We support the the choice of \random  division strategy by showing that the corresponding unigram and bigram distributions are indeed preserved in the samples. We first show that the expected frequency of a word in any sub-corpus sampled using \random is equal to its probability of occurrence in the original corpus. 
%Using Chebyshev inequality we then bound its deviation from the expected value. 

Let $|\w|_C$ denote the frequency of word $\w$ in a given corpus $C$. Let $P_C(\w)$ be the probability that a randomly drawn out word from $C$ is the word $\w$. Note that the empirical probability of drawing out word $\w$ is equal to the number of occurrences of $\w$ in $C$ divided by the total number of words in $C$.
%Then $\Pr(|\w|_C>0)$ is the probability that the word $\w$ occurs at least once in the corpus $C$. Note that $\Pr(|\w|_C>0)$ is simply the probability distribution of $\w$ in $C$. Let $\mathcal{T}_C$ denote the total word count in corpus $C$. For notational convenience we denote $\Pr(|\w|_C>0)$ by $P_C(\w)$. 
We prove the following theorem.
\begin{theorem}
For any sub-corpus $C'$ drawn from the original corpus $C$ using \random and any word , $\w$ we have 
$$\E\left( |\w|_{C'} \over \mathcal{T}_{C'} \right) = P_C(w)$$.
\end{theorem}
\begin{proof}
First we model the probability of the sub-corpus $C'$. Let $x$ and $y$ be random variables  such that the frequency of a word $|\w|_{C'} =x$ and $\mathcal{T}_{C'}=y$. Let the total number of sentences in $C$ be $N$ and in $C'$ be $uN$. Then the probability of the corpus $C'$ with $x$ occurrences of word $\w$ and $y$ being the total word count is given by
\begin{align*}
&\Pr(C'| |C'|=uN,|\w|_{C'} =x, \mathcal{T}_{C'}=y ) \\ 
& = u^{uN} \Pr(\mathcal{T}_{C'}=y) {y \choose x} (P_C(w))^x (1-P_C(w))^{y-x}, 
\end{align*}
where the first term $u^{un}$ is the probability of drawing out $uN$ sentences of sub-corpora  $C'$ from $C$. Now
\begin{align*}
\E\left( x\over y \right) = & \sum_{x,y} { x \over y } \Pr(C'| |C'|=uN,|\w|_{C'} =x, \mathcal{T}_{C'}=y ) \\
=& \sum_{x,y} { x \over y } {y \choose x} (P_C(w))^x (1-P_C(w))^{y-x}  u^{uN} \Pr(\mathcal{T}_{C'}=y)\\
=& \sum_{x,y} { (y-x+1) \over y  } {y \choose x -1} (P_C(w))^{x-1} (1-P_C(w))^{y-x}\\
& \cdot u^{uN} \Pr(\mathcal{T}_{C'}=y)\\
=&{ P_C(w) \over 1-P_C(w) }  \cdot \bigg( \sum_{x,y}  {y \choose x -1}(P_C(w))^{x-1} (1-P_C(w))^{y-x+1}  \\
& \cdot  u^{uN} \Pr(\mathcal{T}_{C'}=y) + \\
&\sum_{x,y} { x-1 \over y  } {y \choose x -1} (P_C(w))^{x-1} (1-P_C(w))^{y-x+1} \\
& \cdot u^{uN} \Pr(\mathcal{T}_{C'}=y) \bigg) \\
= &{ P_C(w) \over 1-P_C(w) }  \left(1+ \E\left({x \over y}\right) \right) \\
&\Rightarrow \E\left( x\over y \right) = P_C(w)
\end{align*}
\end{proof}

We now prove that as long as $P_C(\w)$ obeys a certain condition, with high probability the word $\w$ exists in at least one sub-corpora. We assume that the word count in each sentence is equal to some constant $\ell$.
\begin{theorem}
Let $u=r/100$ where $r$ is the sampling rate. If
\begin{equation}\label{eq:pw} P_C(w)> 1-(1-u)^{1-u \over \ell u}, \end{equation}
then the expected number of randomly sampled sub-corpora with a missing word $\w$ is equal to $\exp(-O(N))$.
% $$\Pr(\text{word $\w$ is missing in all samples}) {\xrightarrow{N\rightarrow \infty } }0 .$$
\end{theorem}
\begin{proof}
We will show that for arbitrary word $\w$ if $P_C(w)$ obeys Equation~\eqref{eq:pw} the expected number of sub-corpora (sampled using \random from any given corpus) is exponential small in size of the original Corpus $N$. Let $X$ be the random variable denoting the total number of sub-corpora of size $uN$ in which the word $\w$ is missing.
$$\E(X) = {N \choose uN} u^{\ell uN}   (1-P_C(w))^{\ell uN}.$$
Using Stirling's approximation,
$\sqrt{2\pi x} \left( {x\over e}\right)^x \le x! \le e\sqrt{2\pi x} \left( {x\over e}\right)^x $ we obtain 
$${N \choose uN}\le u^{-uN}\cdot(1-u)^{-(1-u)N} \cdot {\exp(1)\over  \sqrt{2\pi N u(1-u)}}. $$
Denoting $-u \log u -(1-u) \log u$ by $H(u)$ we obtain
\begin{align*}
\E(X)\le &\sum_y \exp(NH(u)) \cdot u^{uN} (1-P_C(w))^{\ell uN} \\
&\le  \exp(NH(u)) \cdot u^{uN}  ((1-P_C(w))^{ \ell un}) \\
& = \exp(O(N (H(u) + u \log u + u \ell \log (1-P_C(w))))
\end{align*}
Now $\E(X)= e^{-O(N)}$ if 
\begin{align*}
& H(u) + u \log u +  u \ell \log (1-P_C(w)) < 0 \\
 & \Rightarrow -(1-u)\log(1-u) + u \ell \log (1-P_C(w)) < 0 \\
 & \Rightarrow 1-P_C(w) < (1-u)^{1-u\over \ell u},
\end{align*}
which implies Equation \eqref{eq:pw}.

% Using Markov's Inequality we have
% $$ \Pr(X\ge 1)\le \E(X) = e^{-O(N)},$$
% thereby completing the proof.
\end{proof}

\section{Extra Experimental Setup Details}
The statistics concerning the \random, \partition and \shuffle approaches and the \baseline model are presented in Table~\ref{tab:hyper}. 
% The models have an associated sampling rate  of $r\%$ associated (i.e. $10\%$), this refers to the data being split into $10$ parts and the actual model being composed of 10 sub-models of size $N/10$ each, where $N$ is the total number of sentences. The hyper-parameters and statistics concerning the \random, \partition and \shuffle approaches and the baseline model are presented in Table~\ref{tab:hyper}.
\begin{table}[ht!]
\footnotesize
\centering
\resizebox{\linewidth}{!}{
\begin{tabular}{lccc}
\hline
Model&Sampling& Min-count  & Vocab. size\\
%& vocab. size \\
&rate& threshold & (common)\\
% & (union)\\
\hline
%\texttt{Baseline}&--&100&307,451\\
\baseline &--&100&300,000\\
\random &10\%&10&187,315\\
\partition &10\%&10&135,548\\
\shuffle &10\%&--&299,790\\
\random &1\%&1&60,848\\
\partition &1\%&1&47,692\\
\shuffle &1\%&--&262,390\\
\hline
\end{tabular}
}
\caption{Statistics of SGNS trained models. The windows size is 10, dimension of each model is 500, count of negative samples is 5, number of iteration is 5 and the all the models or sub-models are calculated using 10 threads.}
\label{tab:hyper}
\end{table}

\begin{figure*}[h!]	
\centering

    \begin{subfigure}{.30\linewidth}
  		\includegraphics[width=\linewidth]{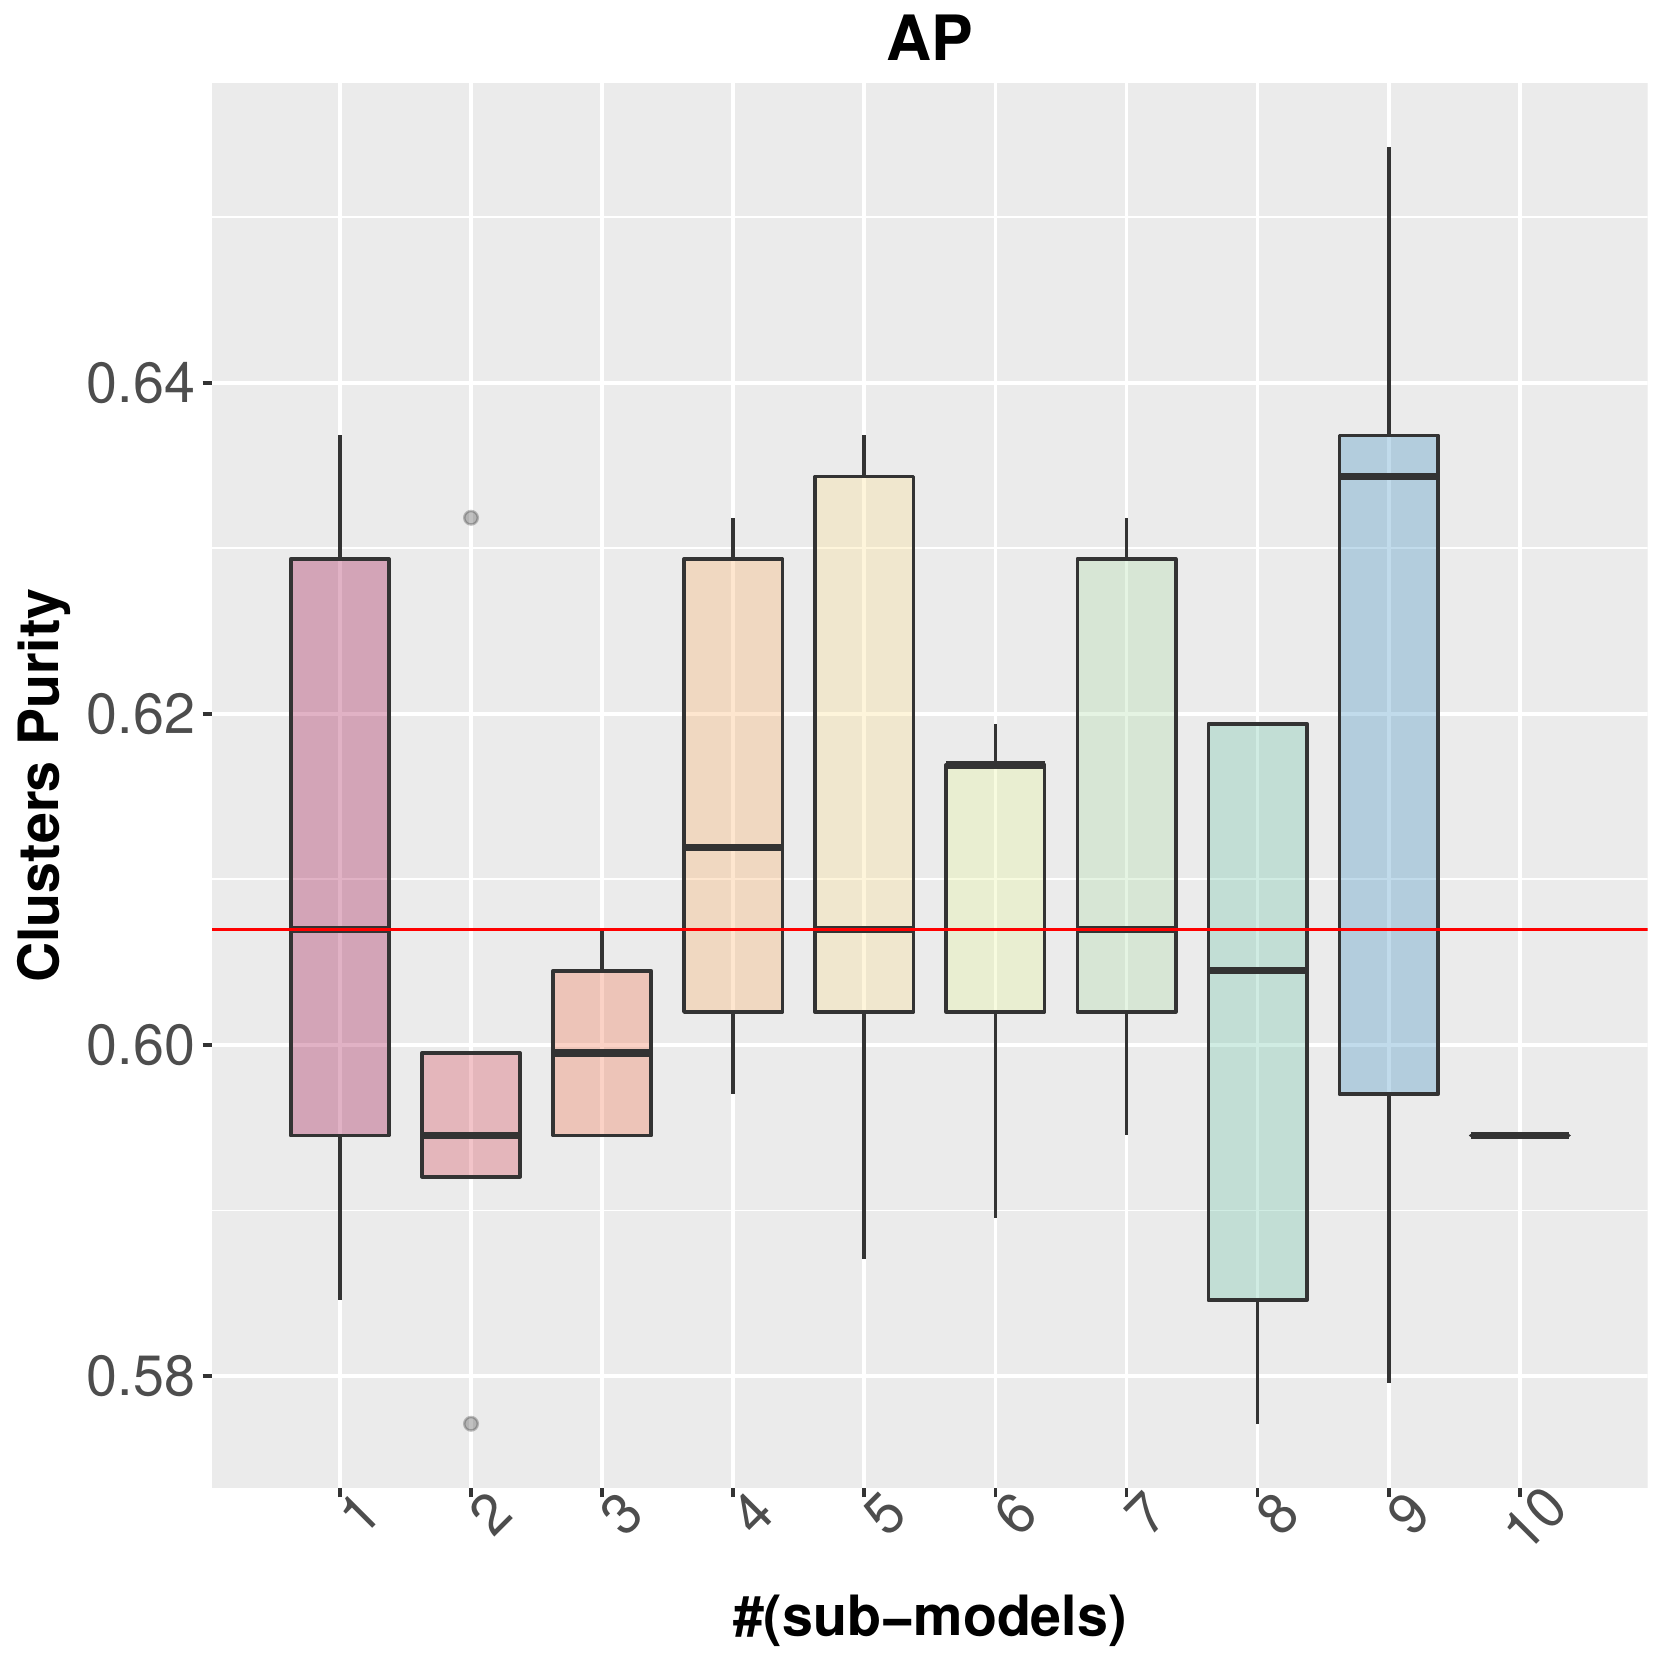}
    \end{subfigure}
    \begin{subfigure}{.30\linewidth}
  		\includegraphics[width=\linewidth]{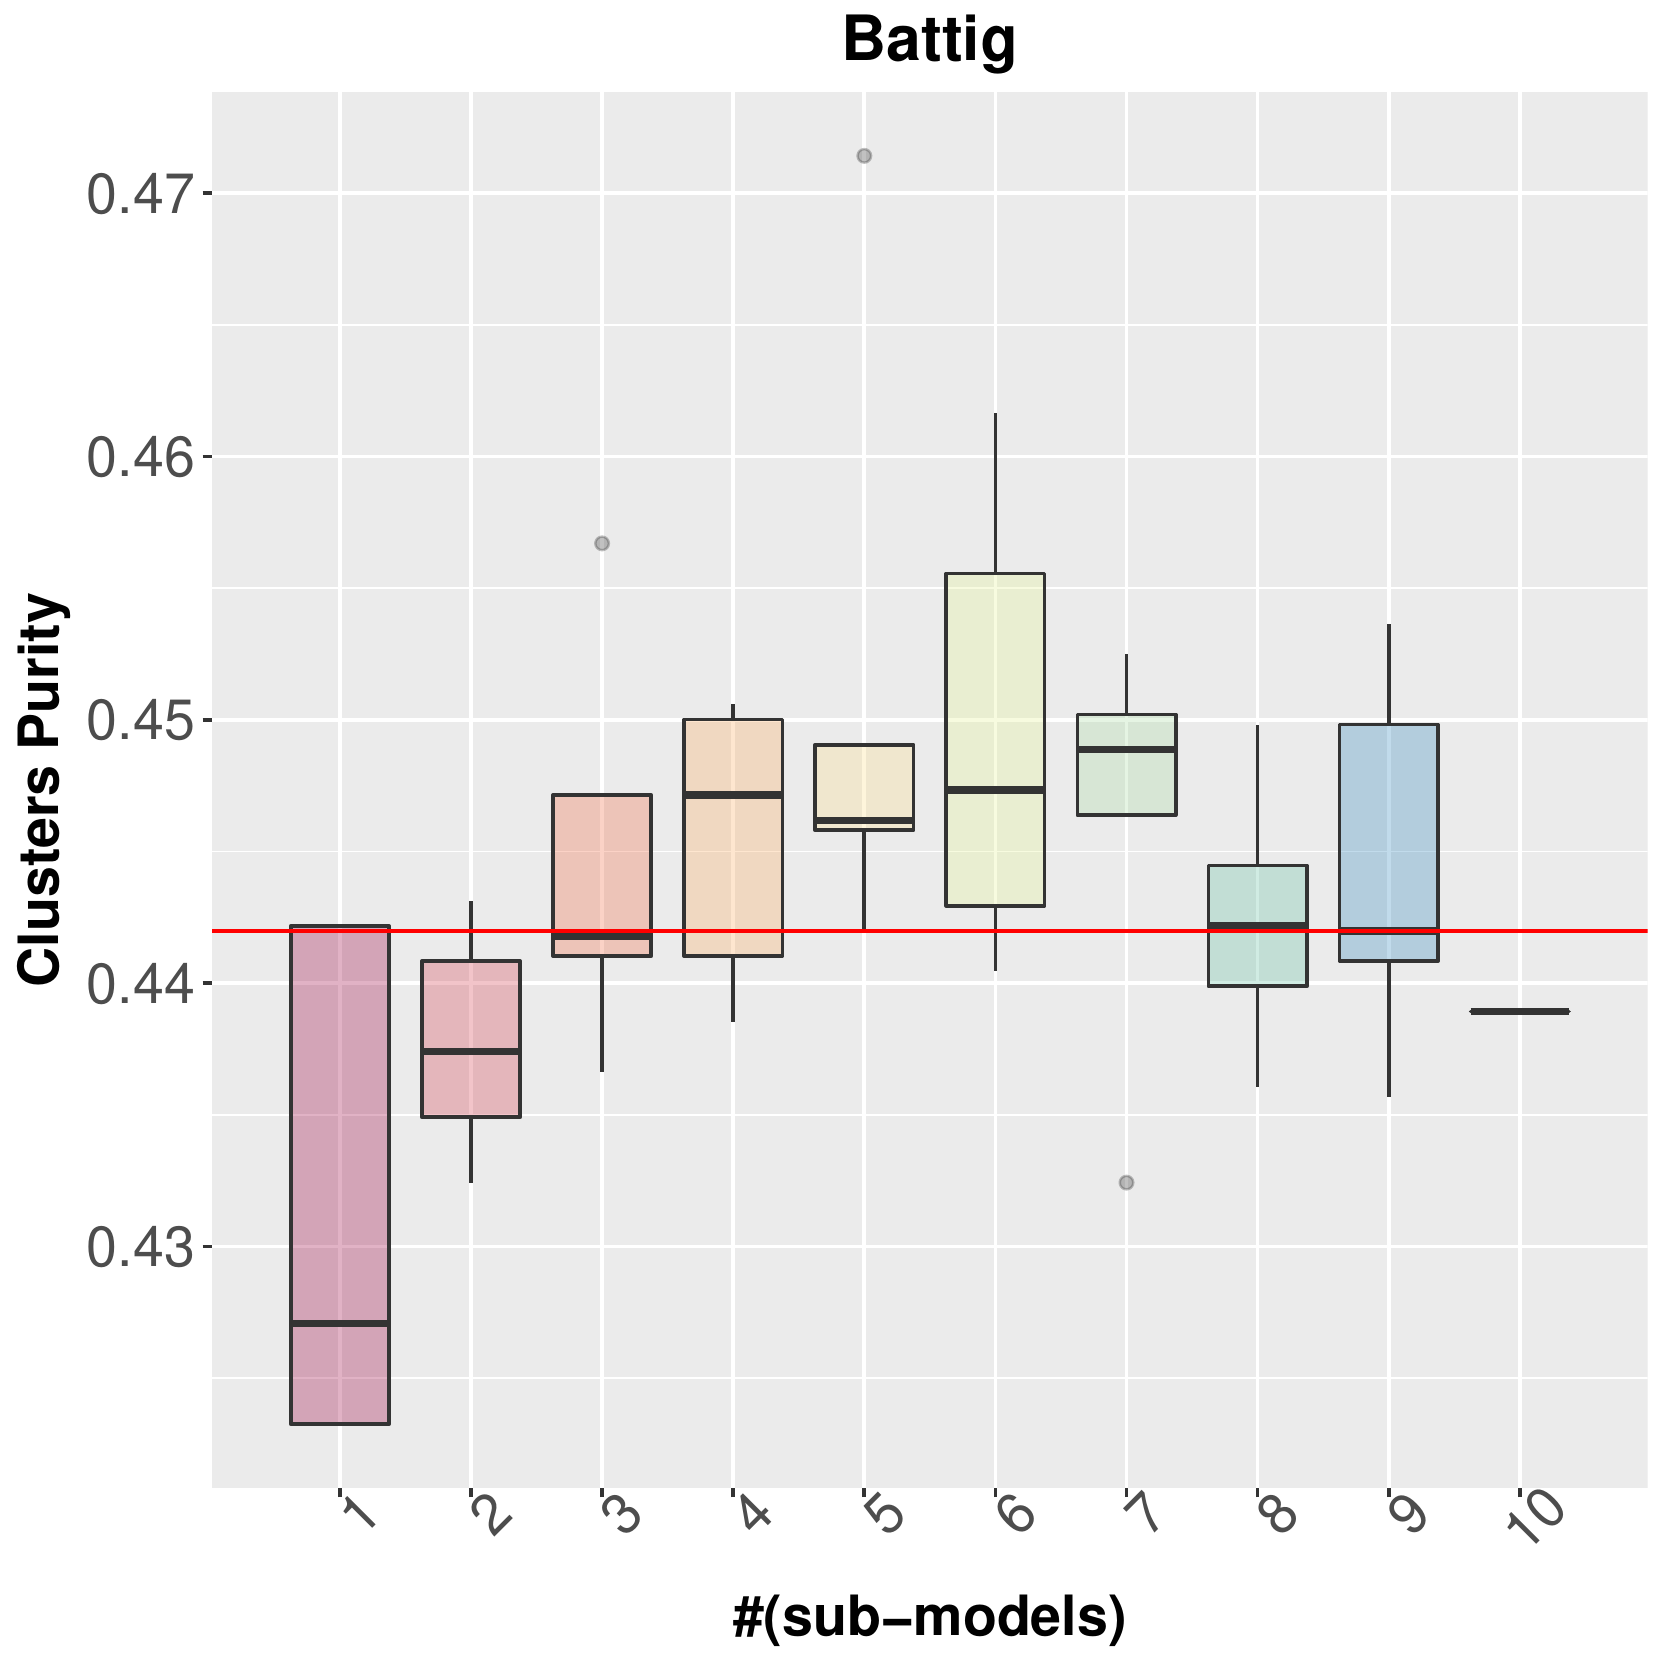}
    \end{subfigure}
    \begin{subfigure}{.30\linewidth}
  		\includegraphics[width=\linewidth]{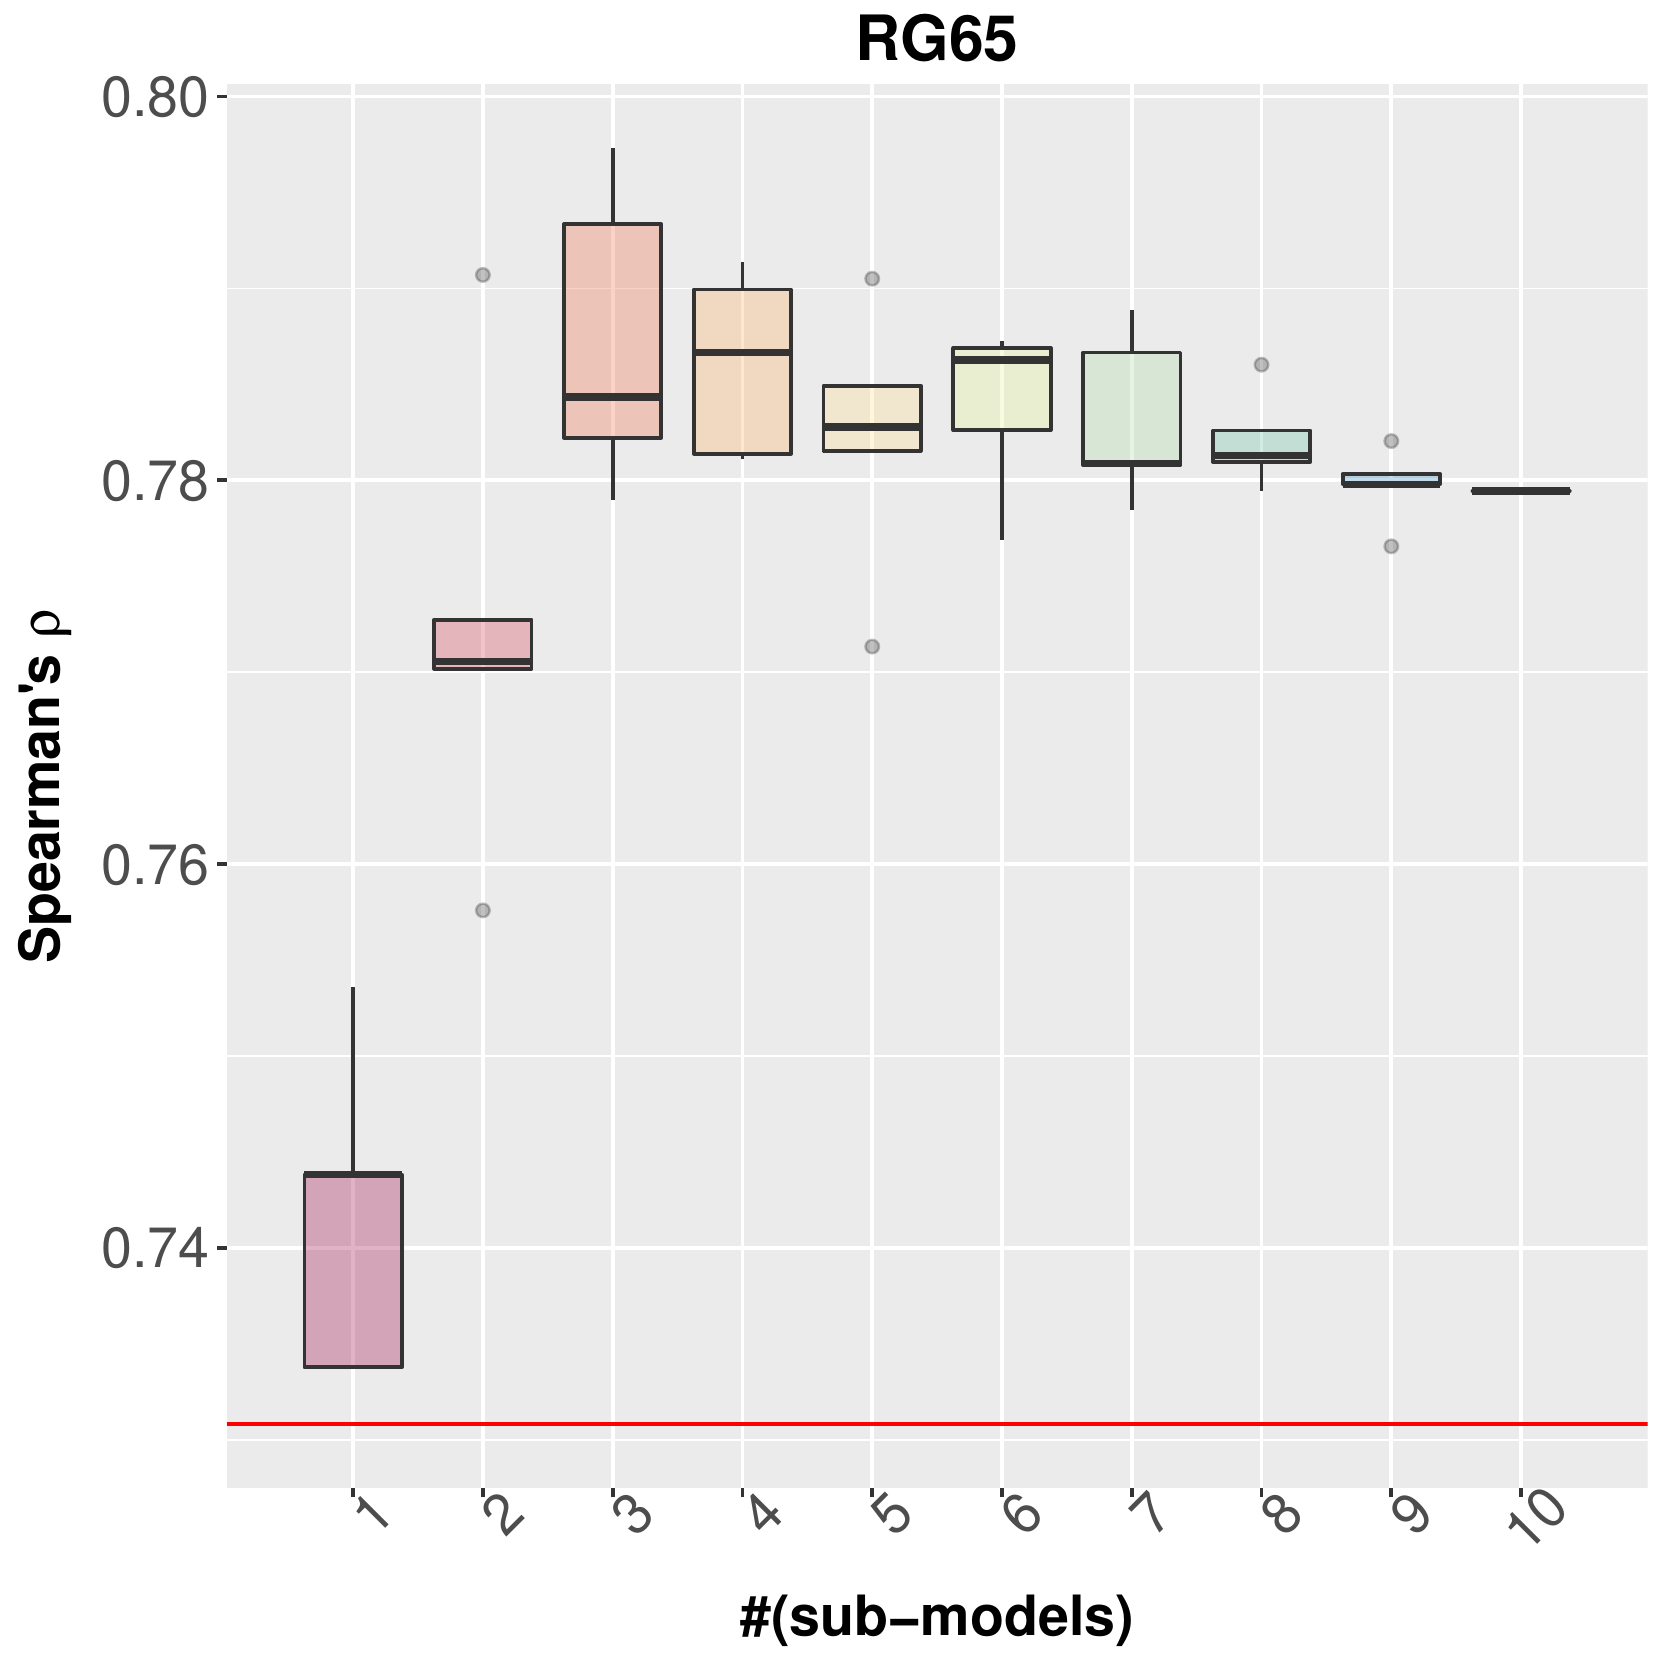}
    \end{subfigure}
	\begin{subfigure}{.30\linewidth}
  		\includegraphics[width=\linewidth]{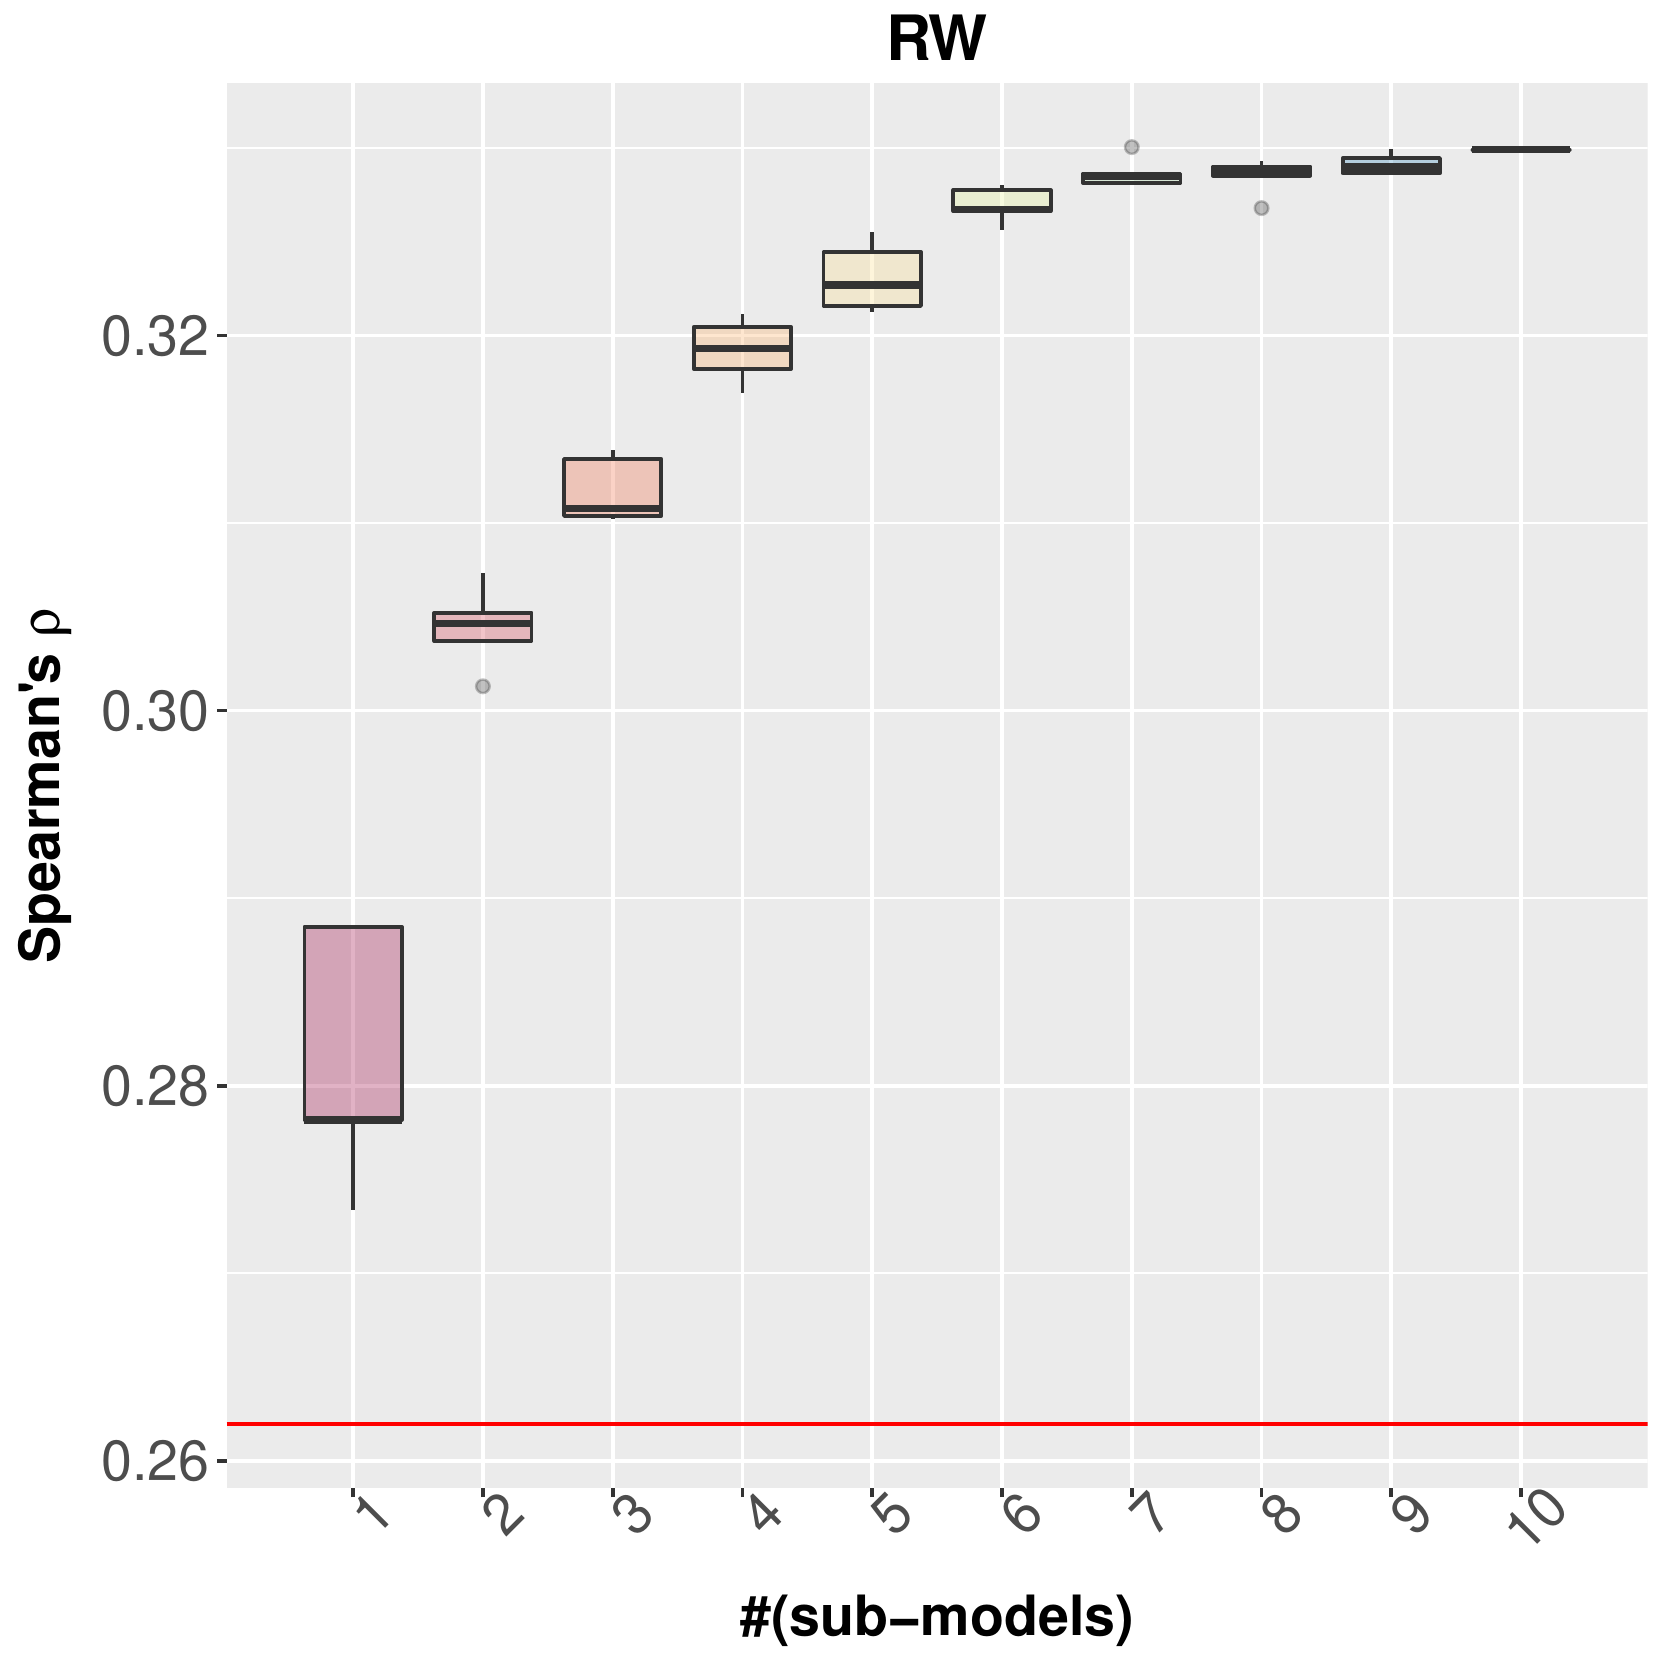}
	\end{subfigure}
    \begin{subfigure}{.30\linewidth}
  		\includegraphics[width=\linewidth]{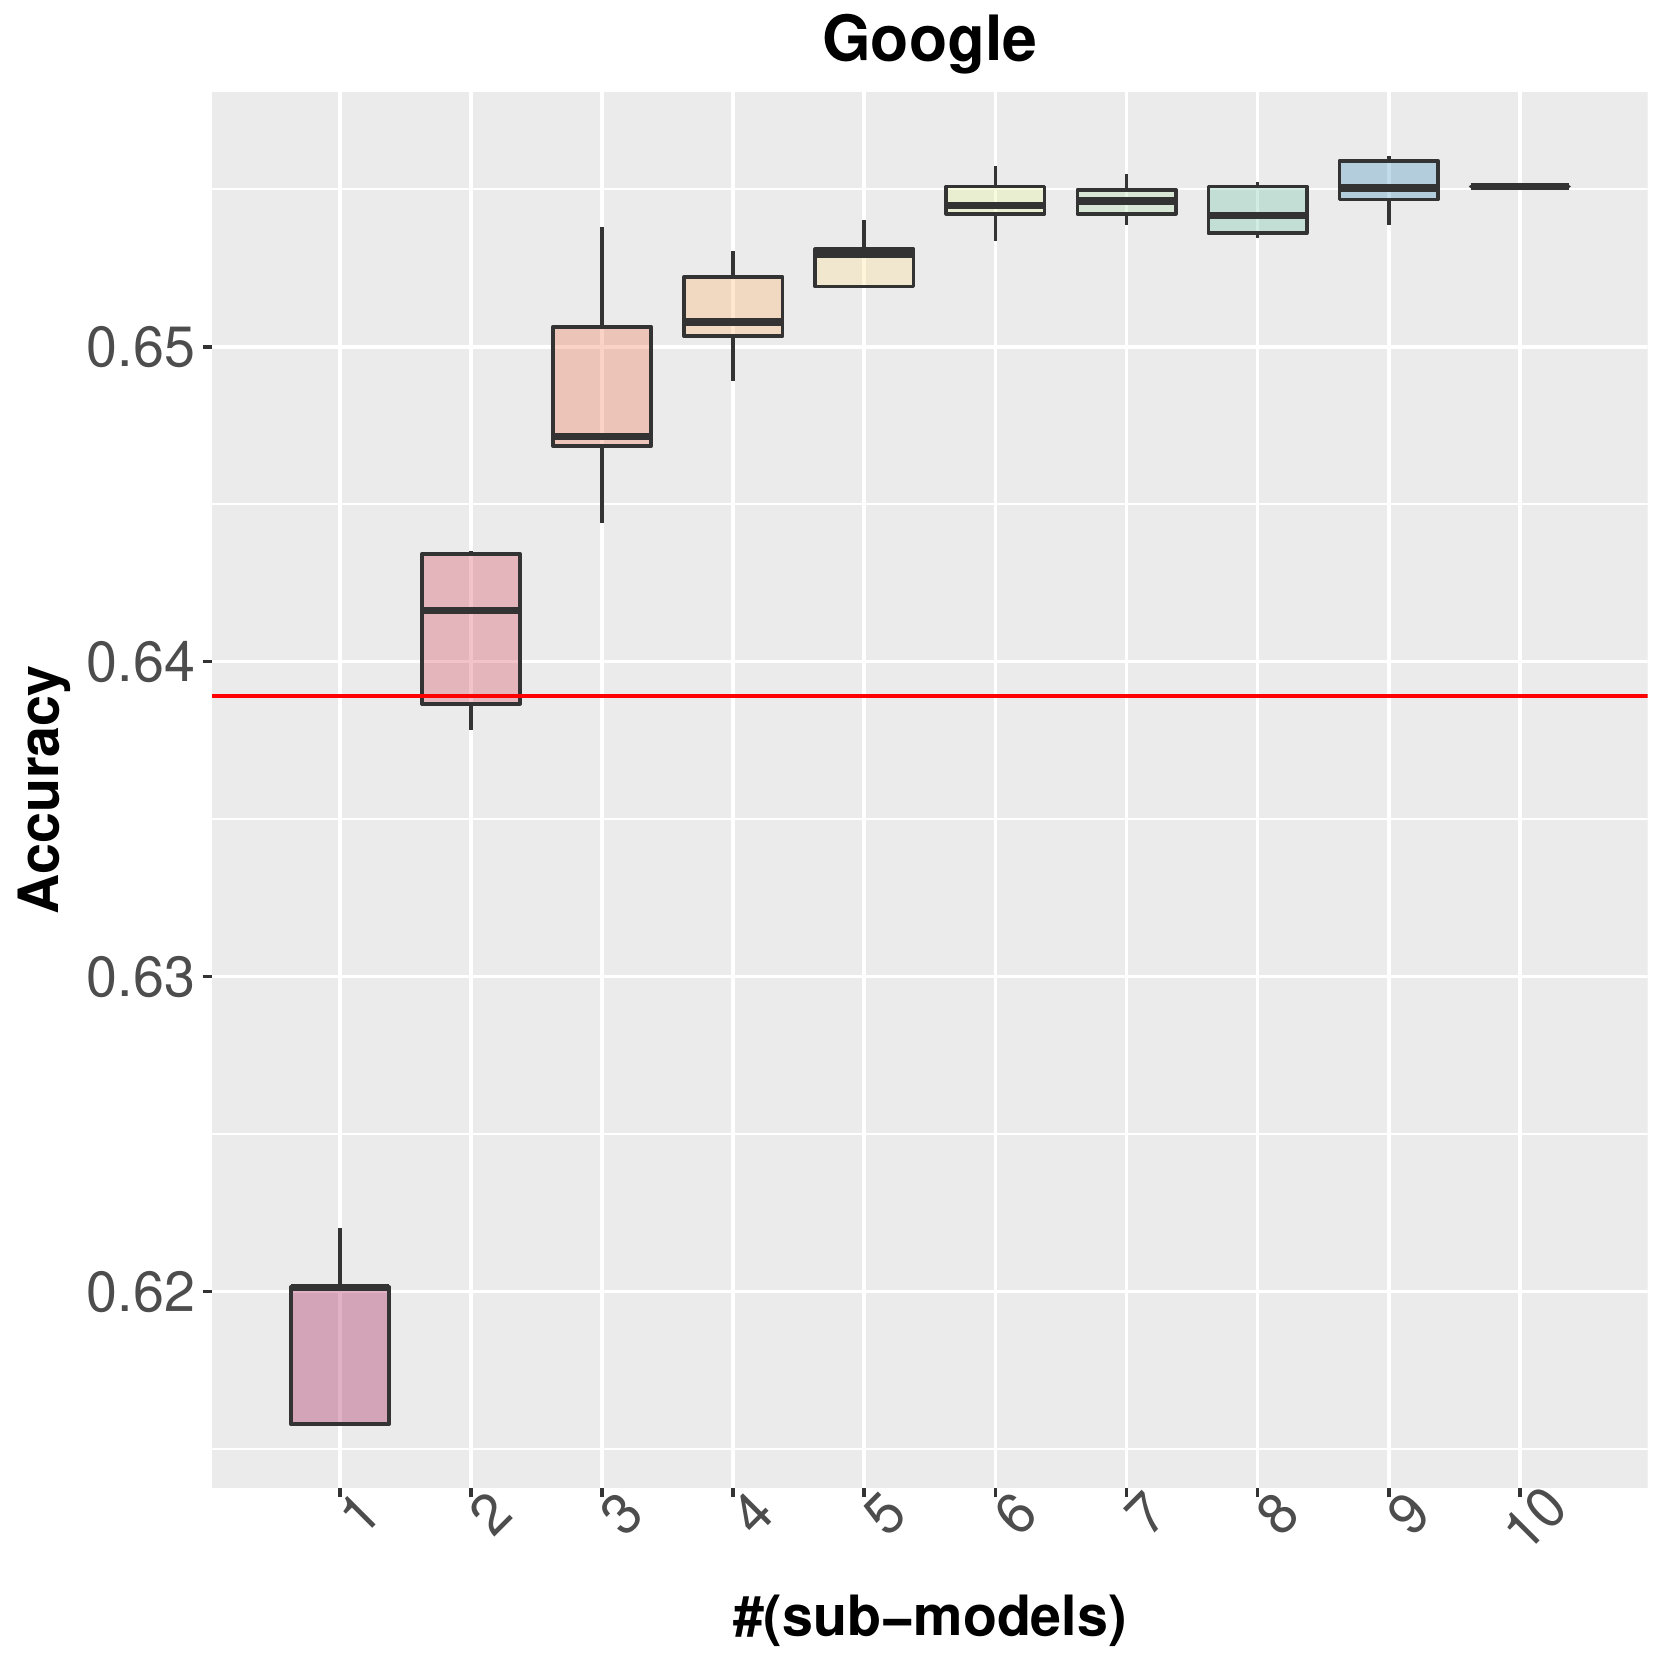}
    \end{subfigure}
    \begin{subfigure}{.30\linewidth}
  		\includegraphics[width=\linewidth]{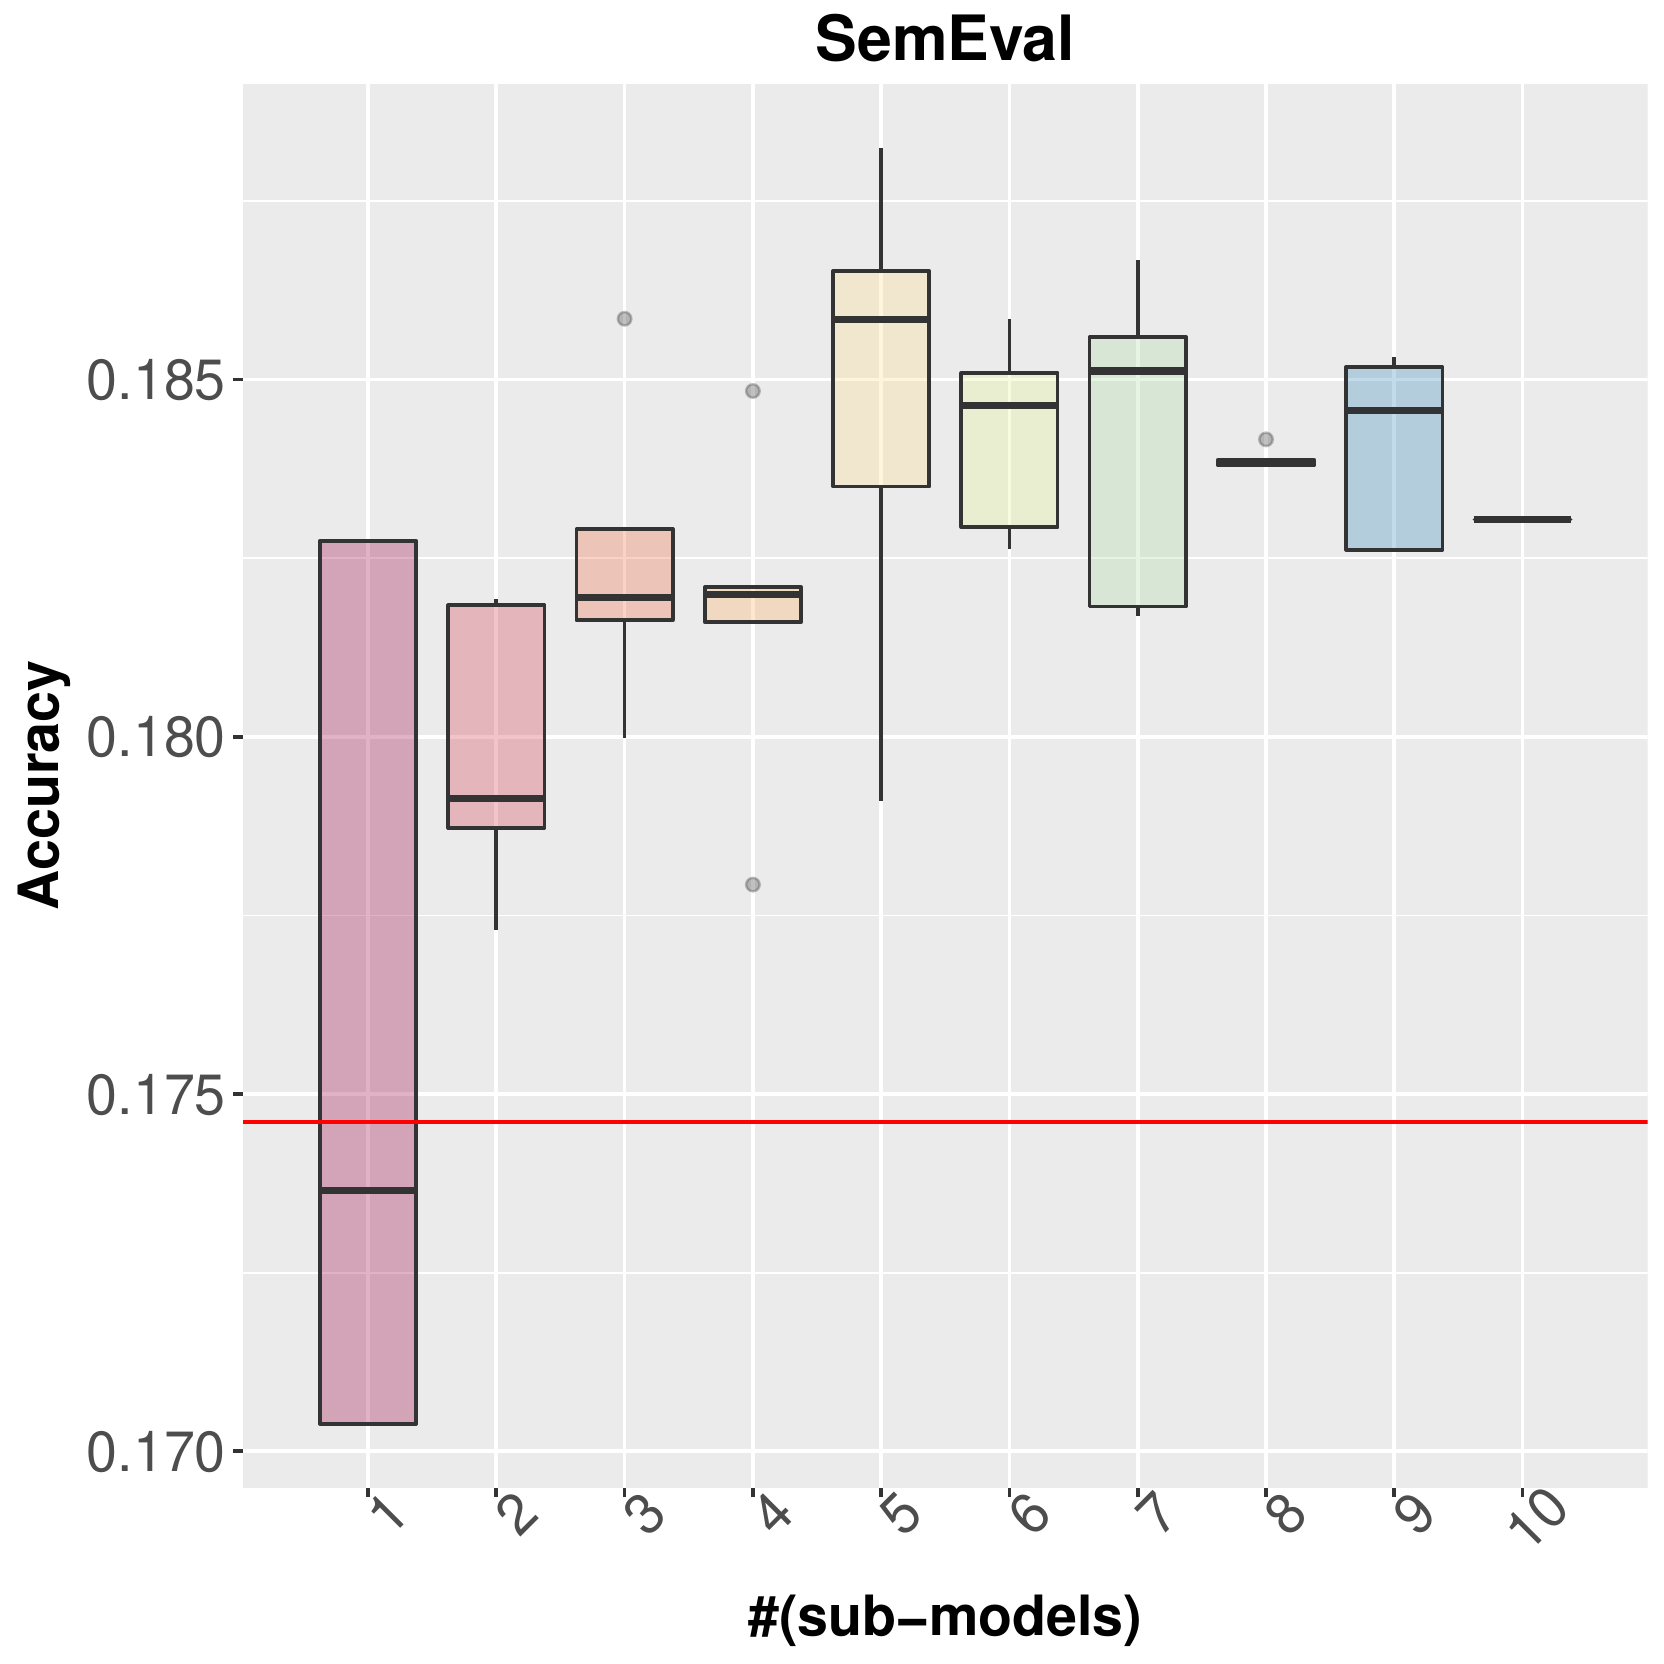}
    \end{subfigure}

	\caption{Box Plots showing the effectiveness of merging Sub-Models with the \texttt{Shuffle + \problem} approach. \problem initialized with PCA (Epochs = $3$, Sample Rate = $10\%$, Dimensions = $500$). The red line indicates the \baseline   performance. Top and bottom of the boxes represent one quartile above and below the mean. The whiskers on top of and under the boxes represent the highest and the lowest values that are within the 1.5 IQR (interquartile range) of the upper and lower quartile. Dots are outliers that are even higher or lower than the ends of whiskers.}
	\label{fig:n-10-box}
\end{figure*}

While merging using \pca, we used the TruncatedSVD implementation provided in scikit-learn~\footnote{http://scikit-learn.org}. For the matrix transformations in \problem we used the orthogonal\_procrustes method provided in SciPy (scipy.linalg.orthogonal\_procrustes). Both of these Python modules support BLAS acceleration. Note that using orthogonal Procrustes is considerably slower since SVD is performed multiple times as opposed to once for PCA. Additionally, \problem is run for multiple epochs.

\begin{figure*}[ht!]
	\centering
	
    \begin{subfigure}{.24\linewidth}
    	\centering
  		\includegraphics[width=\linewidth]{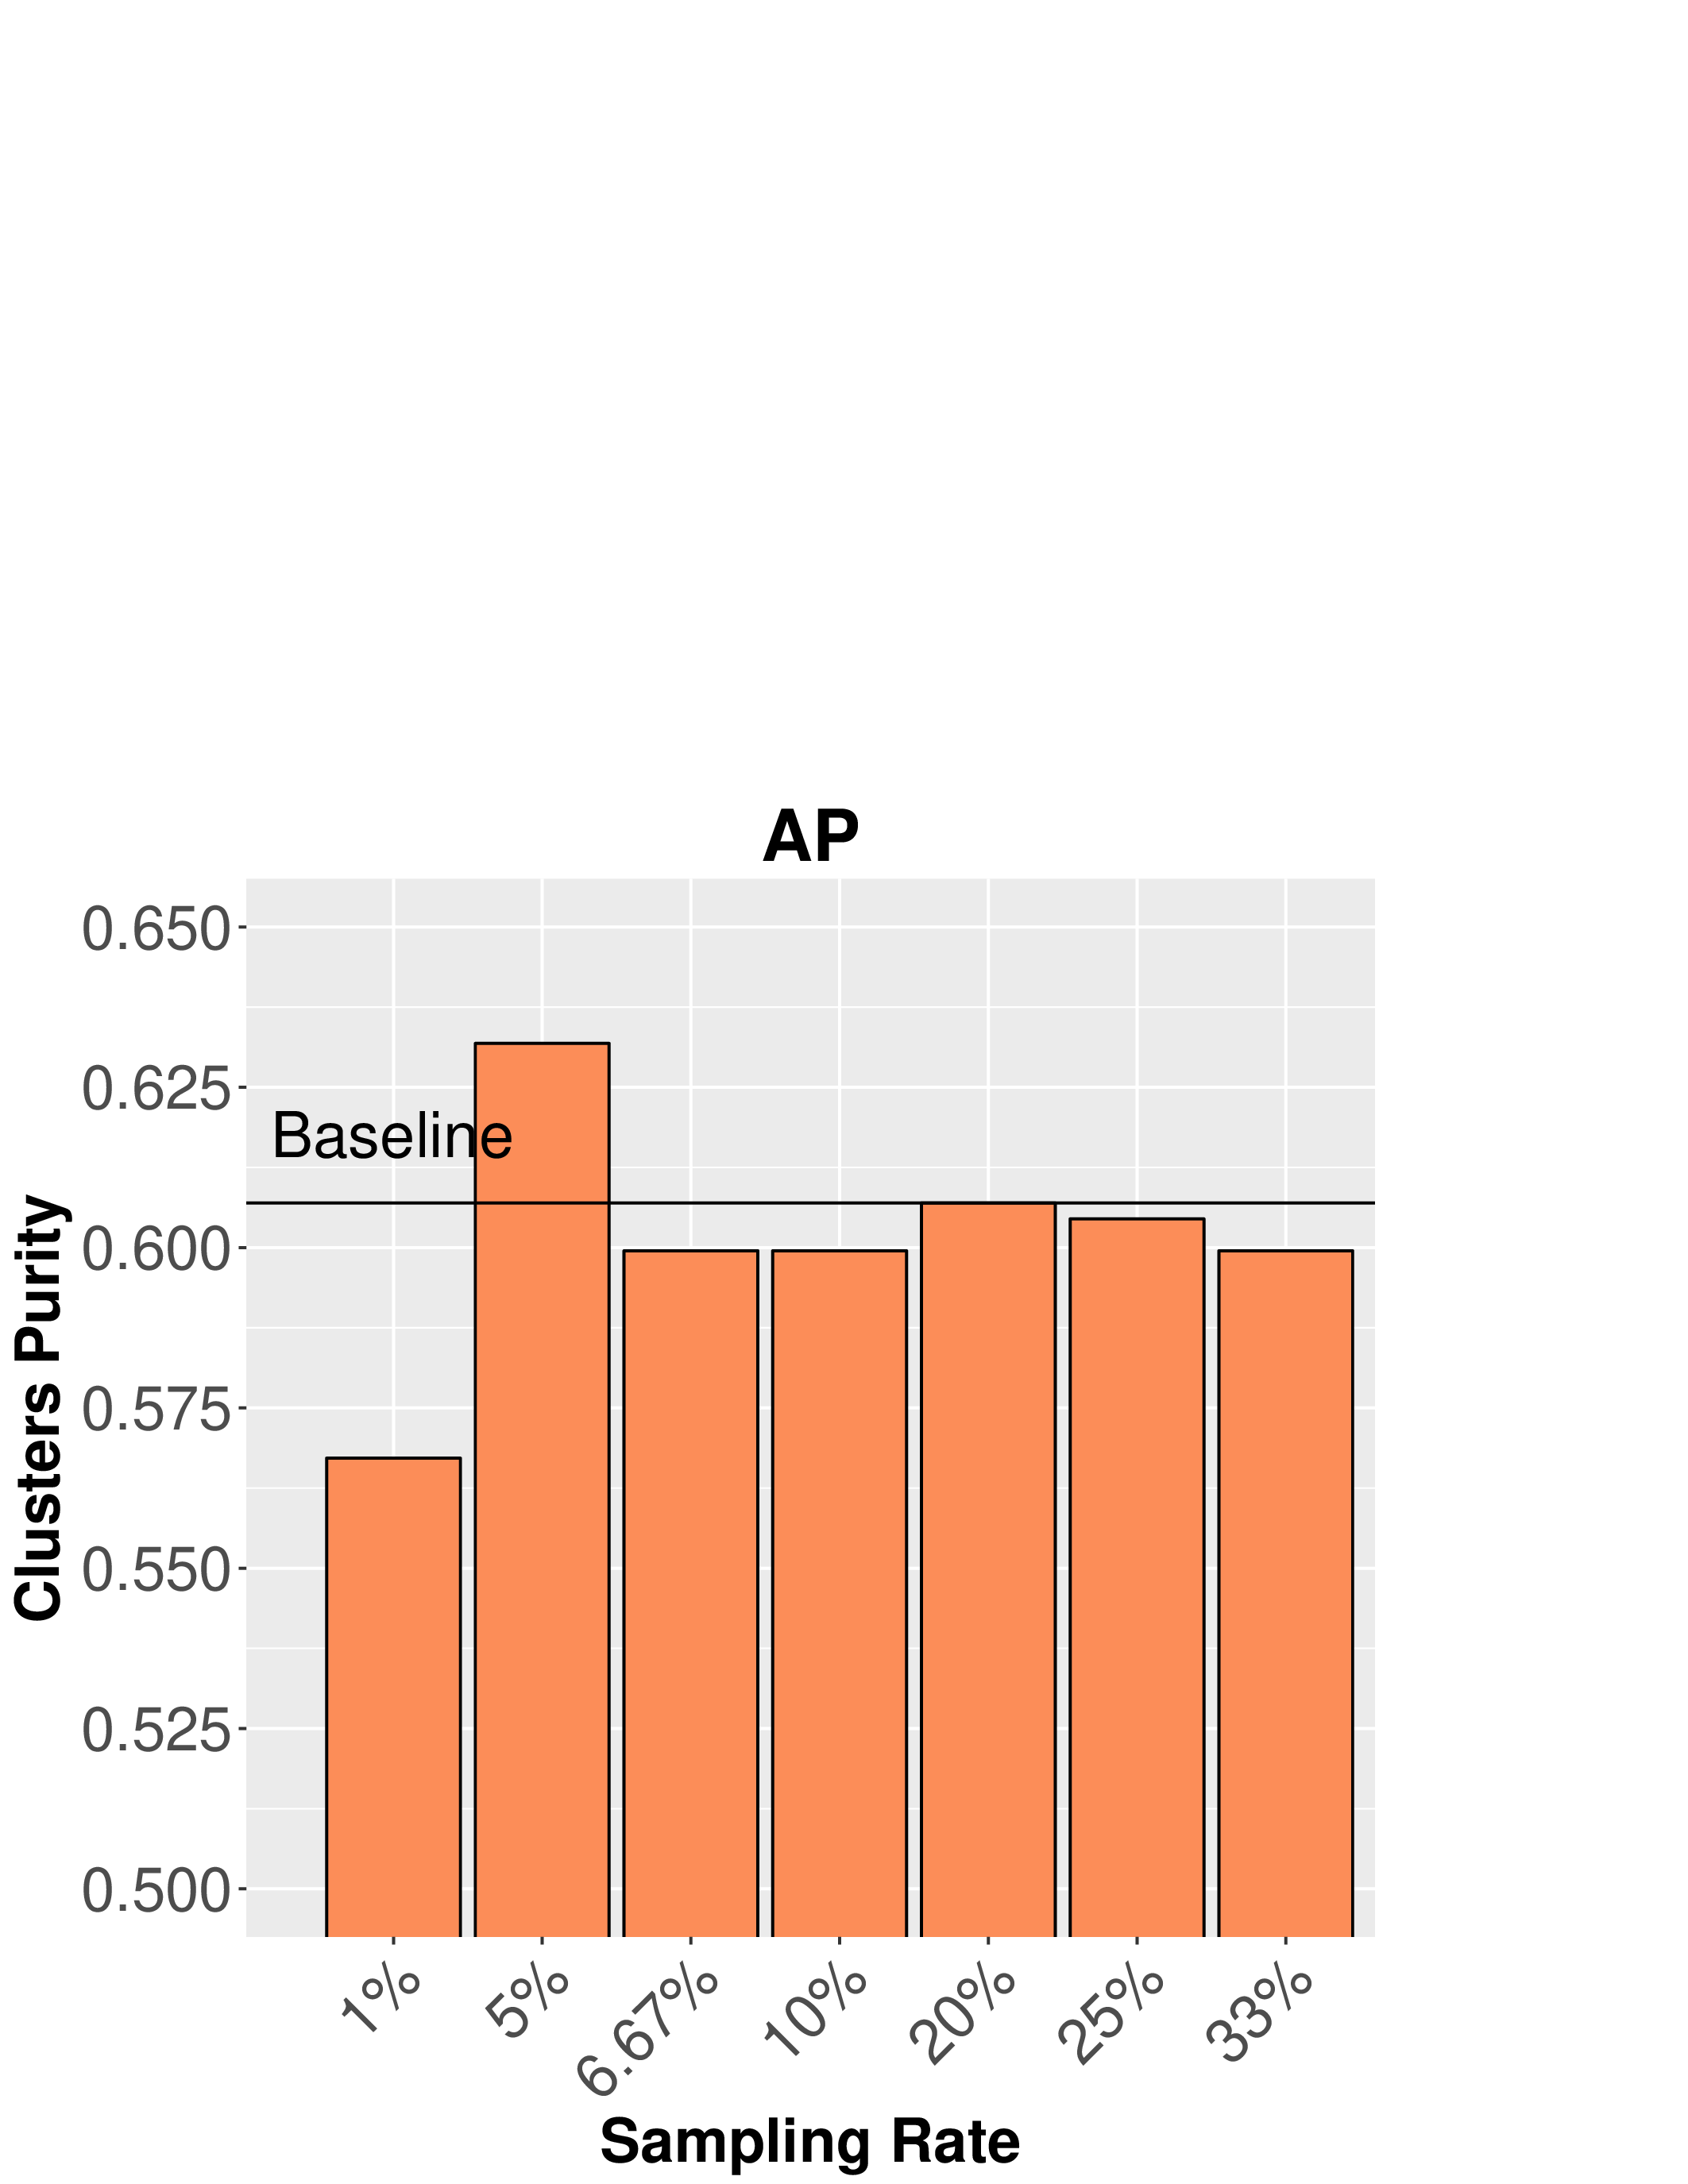}
    \end{subfigure}
    \begin{subfigure}{.24\linewidth}
    	\centering
  		\includegraphics[width=\linewidth]{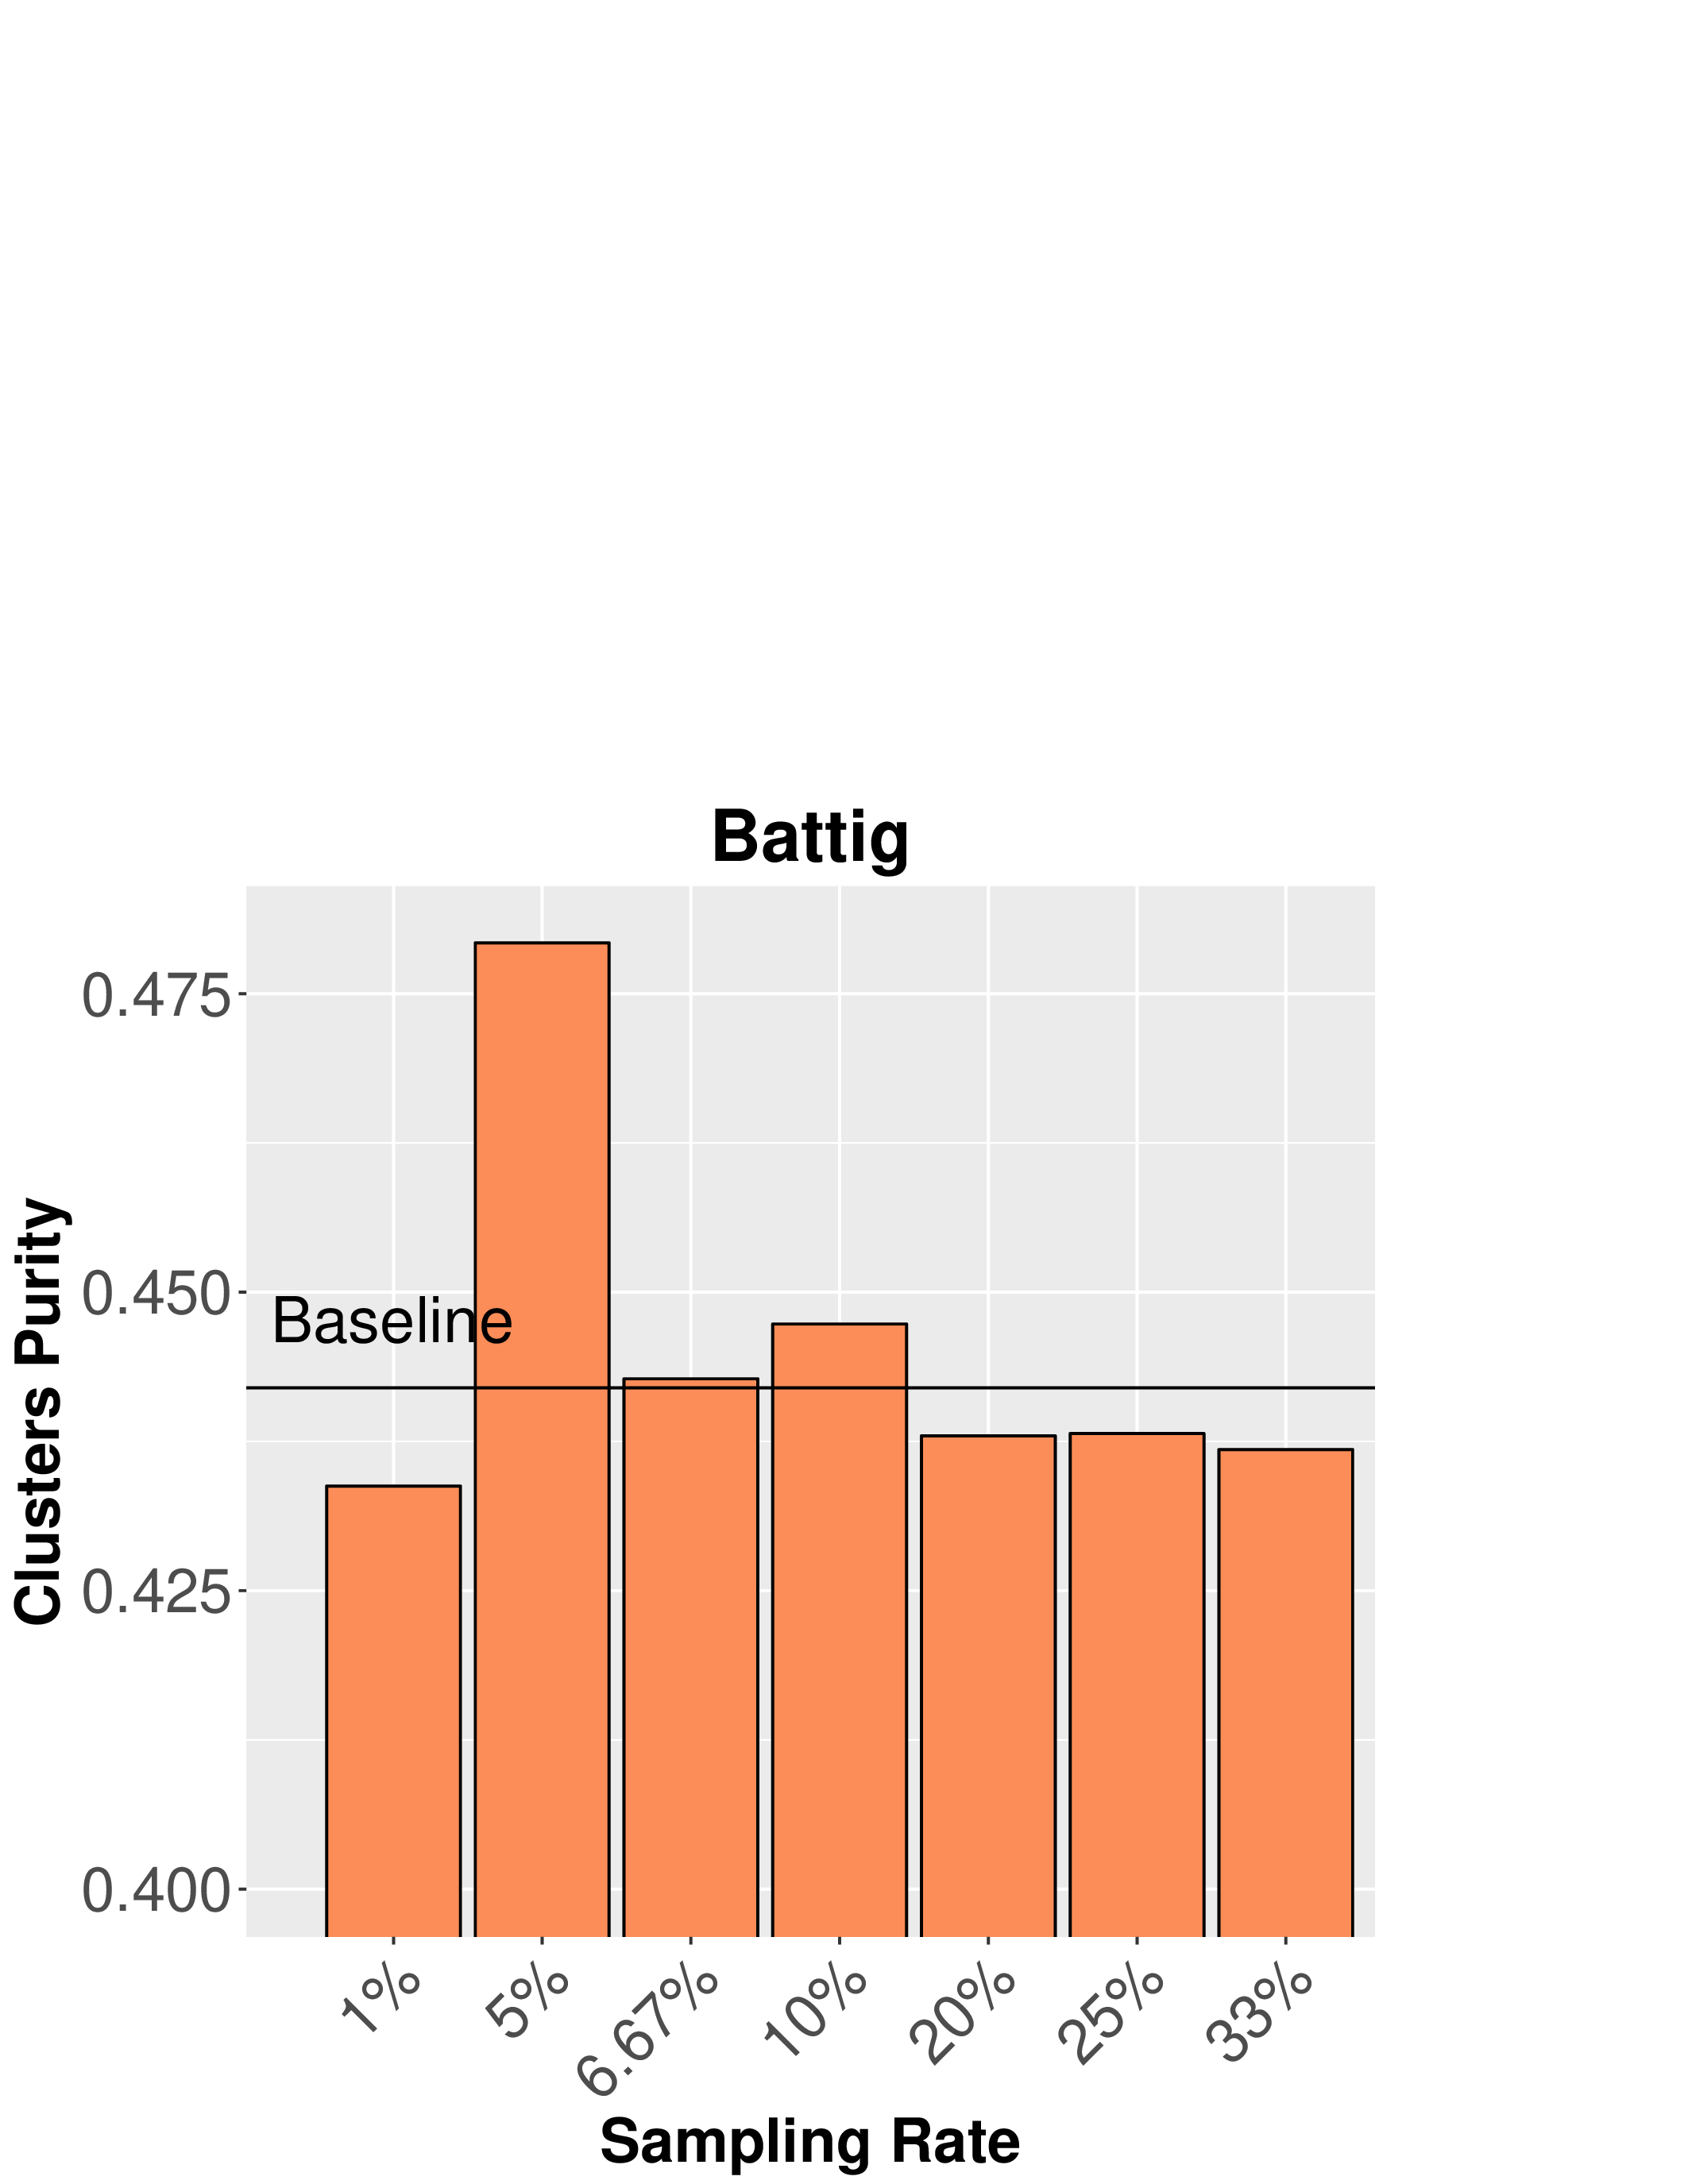}
    \end{subfigure}
    \begin{subfigure}{.24\linewidth}
        \centering
  		\includegraphics[width=\linewidth]{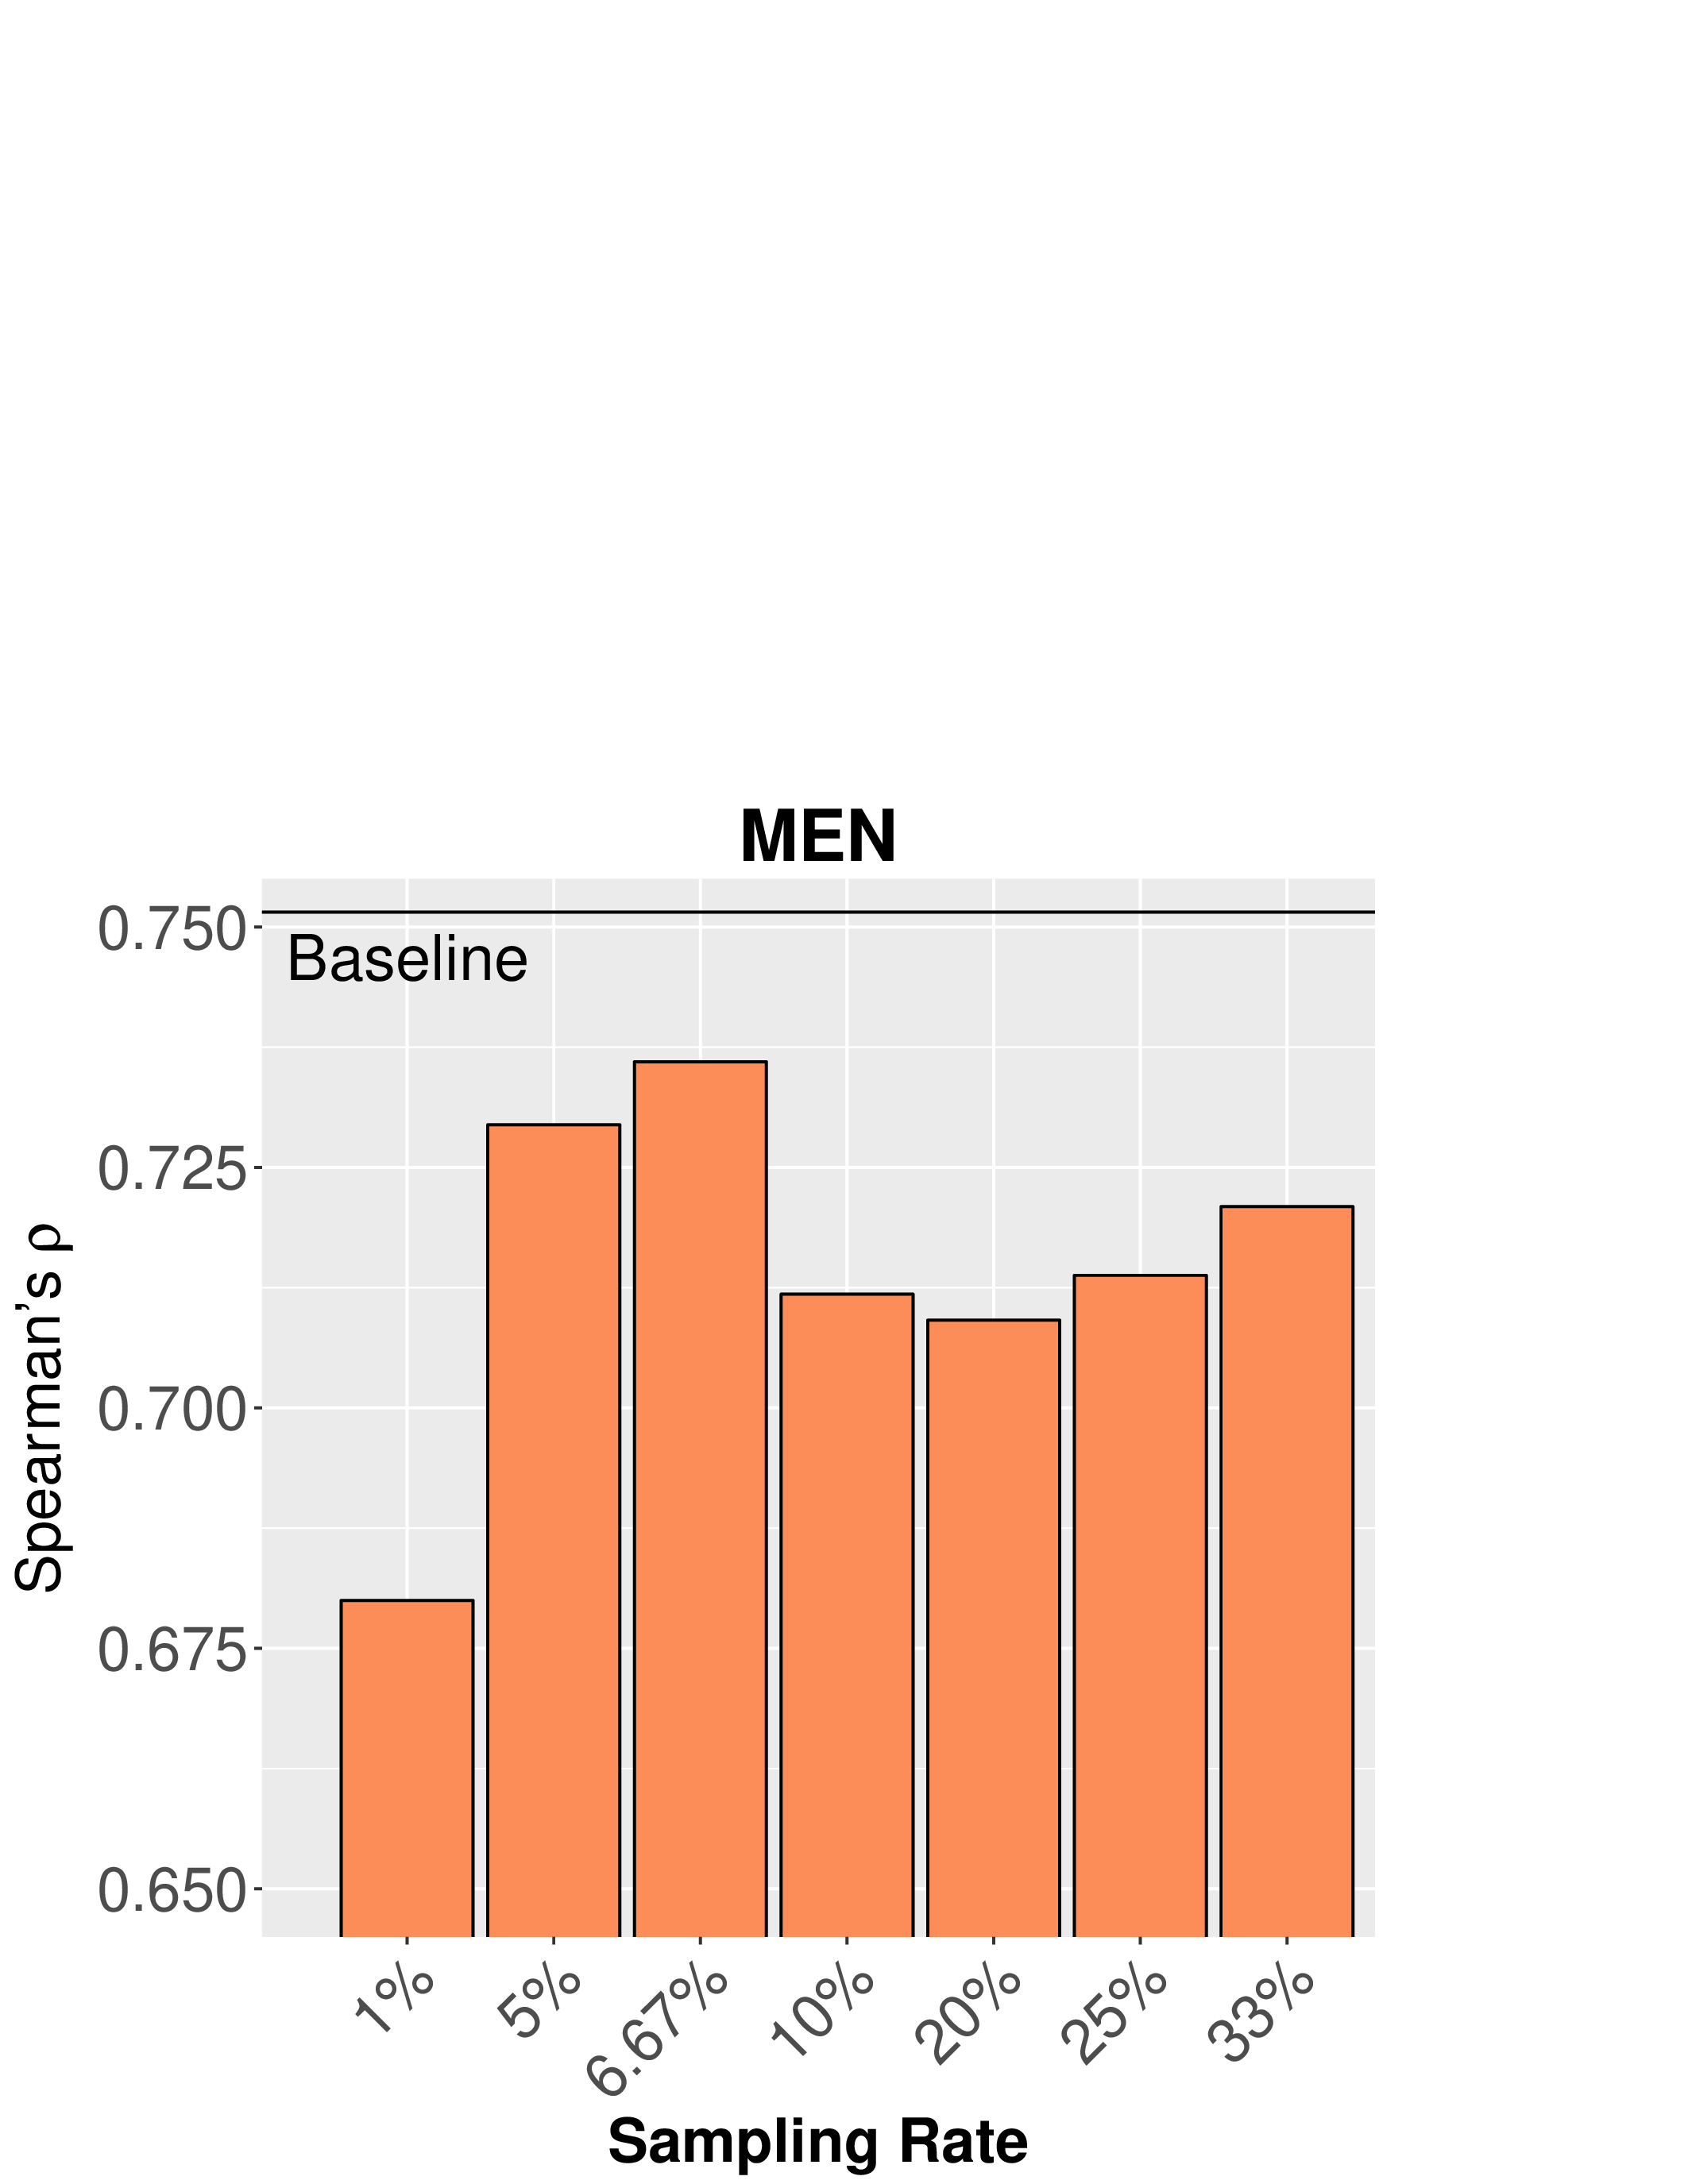}
    \end{subfigure}
    \begin{subfigure}{.24\linewidth}
    	\centering
  		\includegraphics[width=\linewidth]{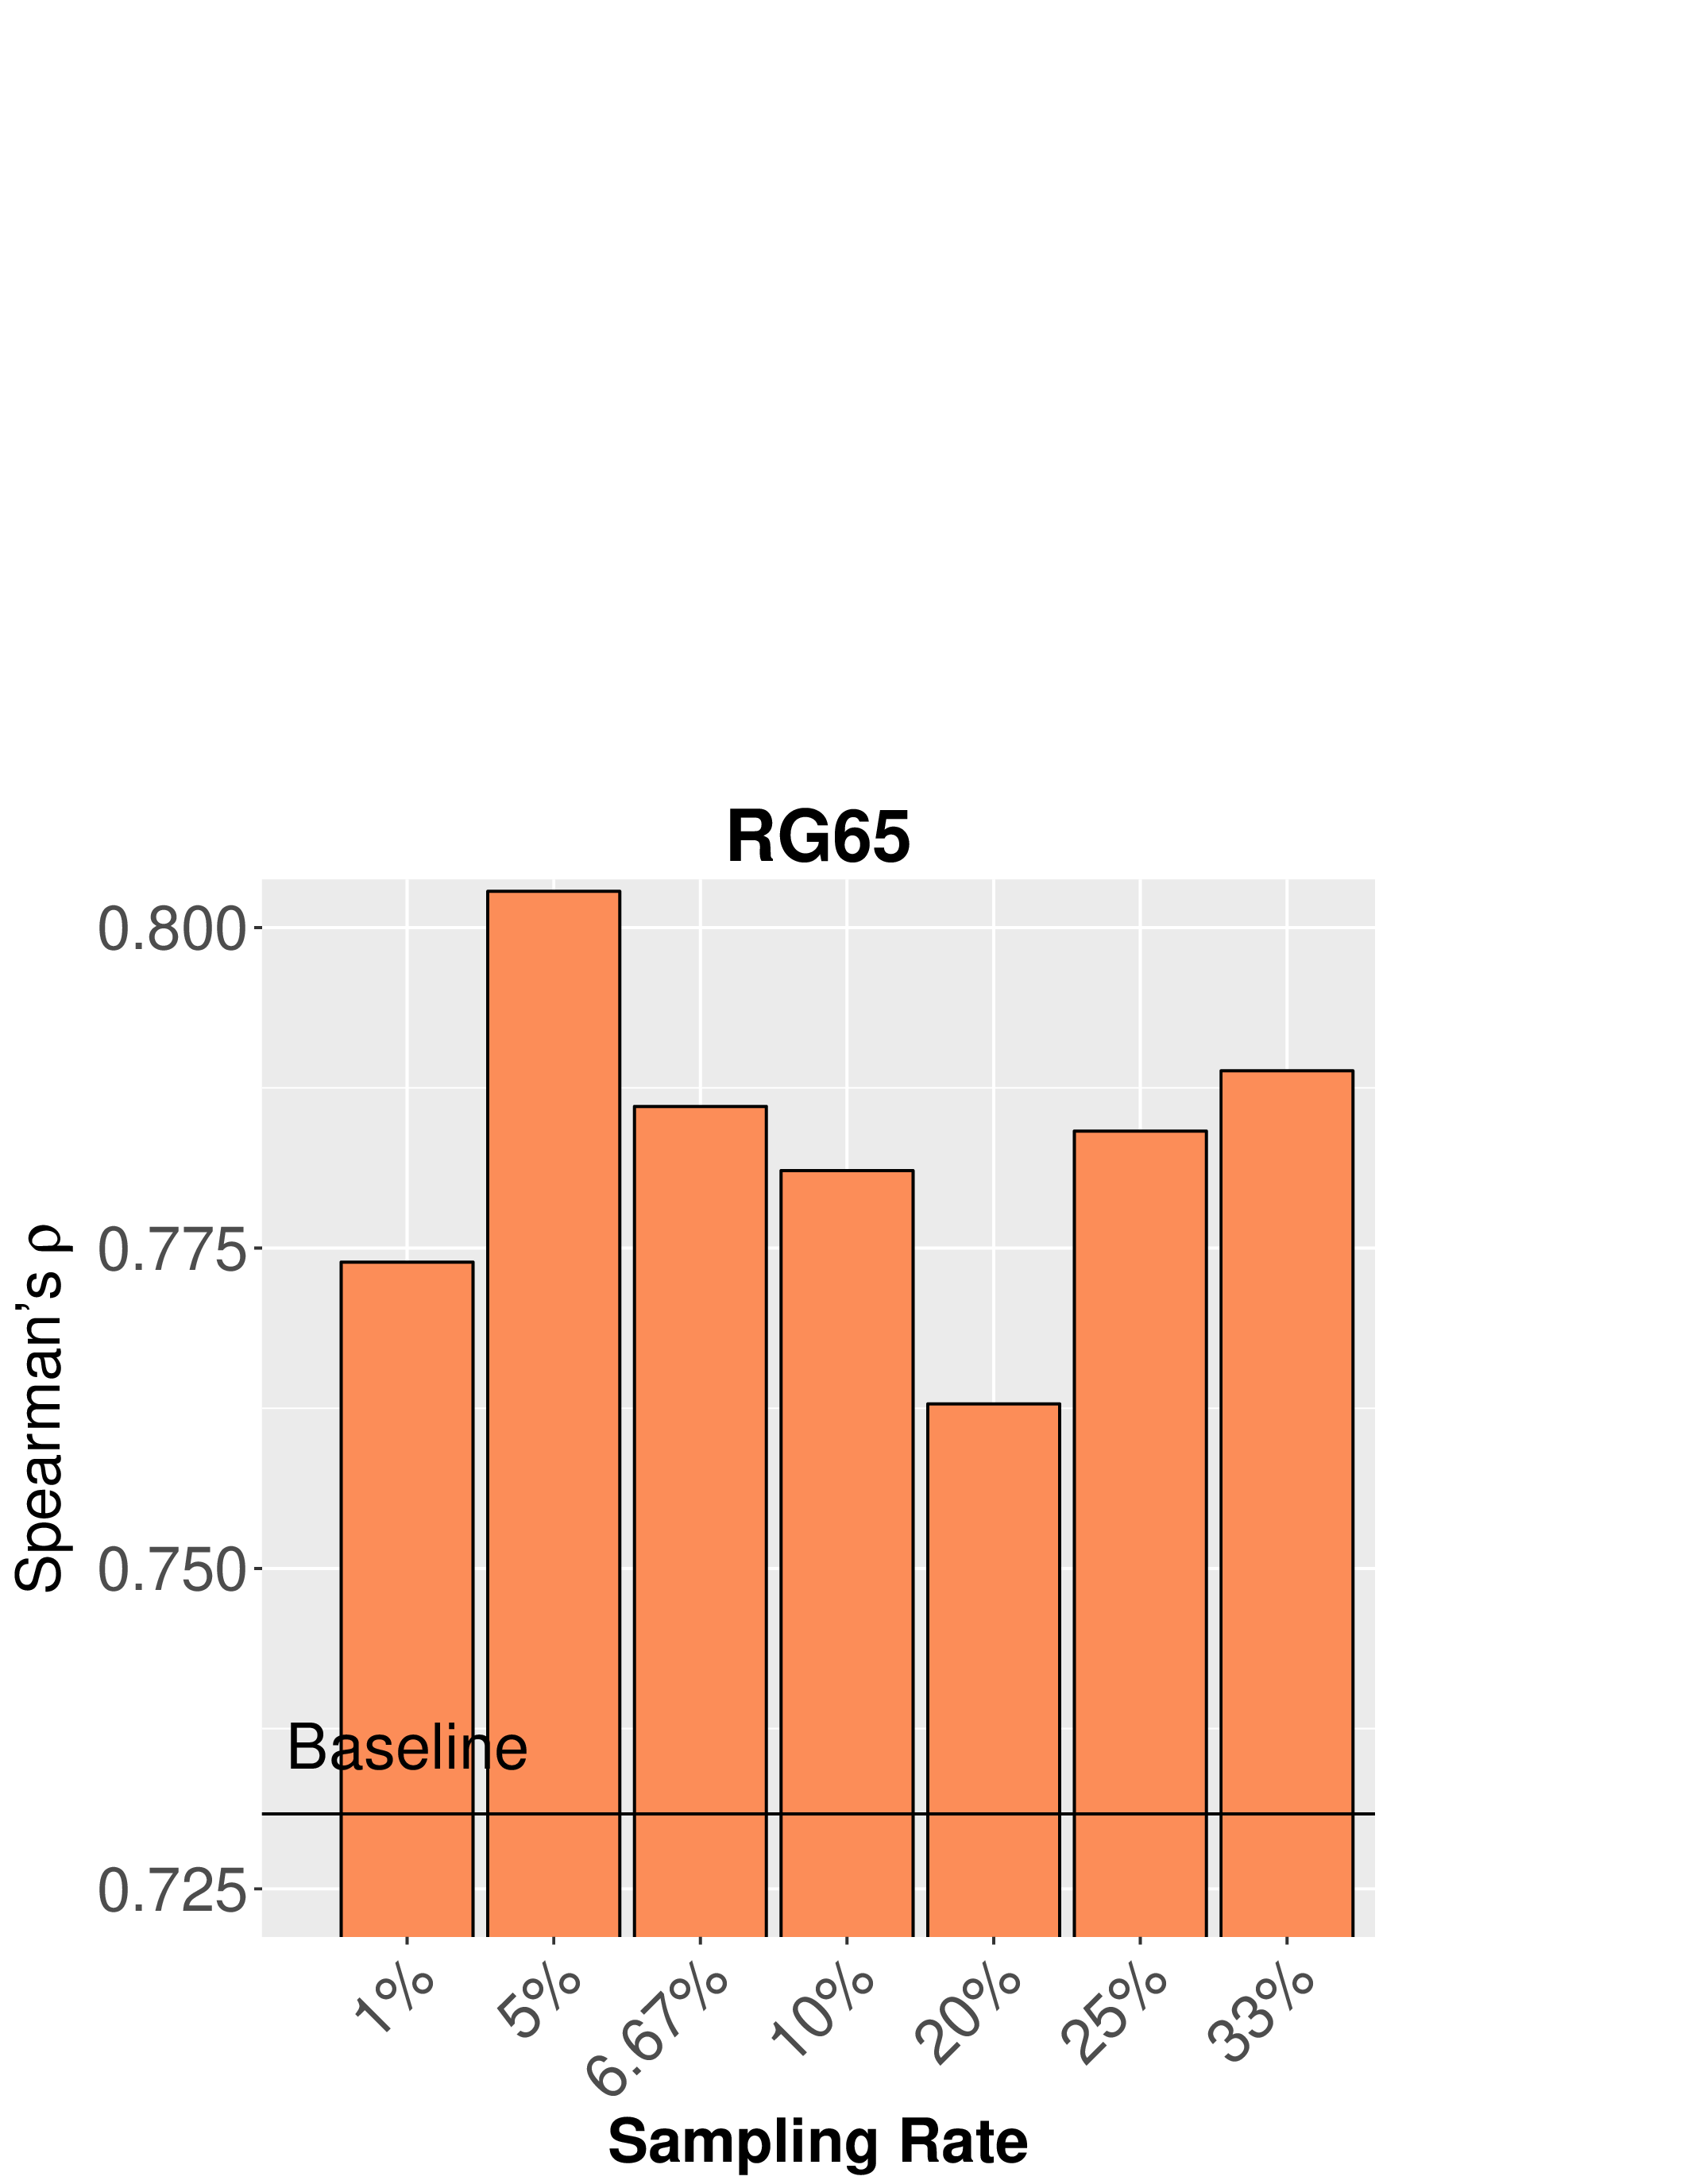}
    \end{subfigure}
	\begin{subfigure}{.24\linewidth}
    	\centering
  		\includegraphics[width=\linewidth]{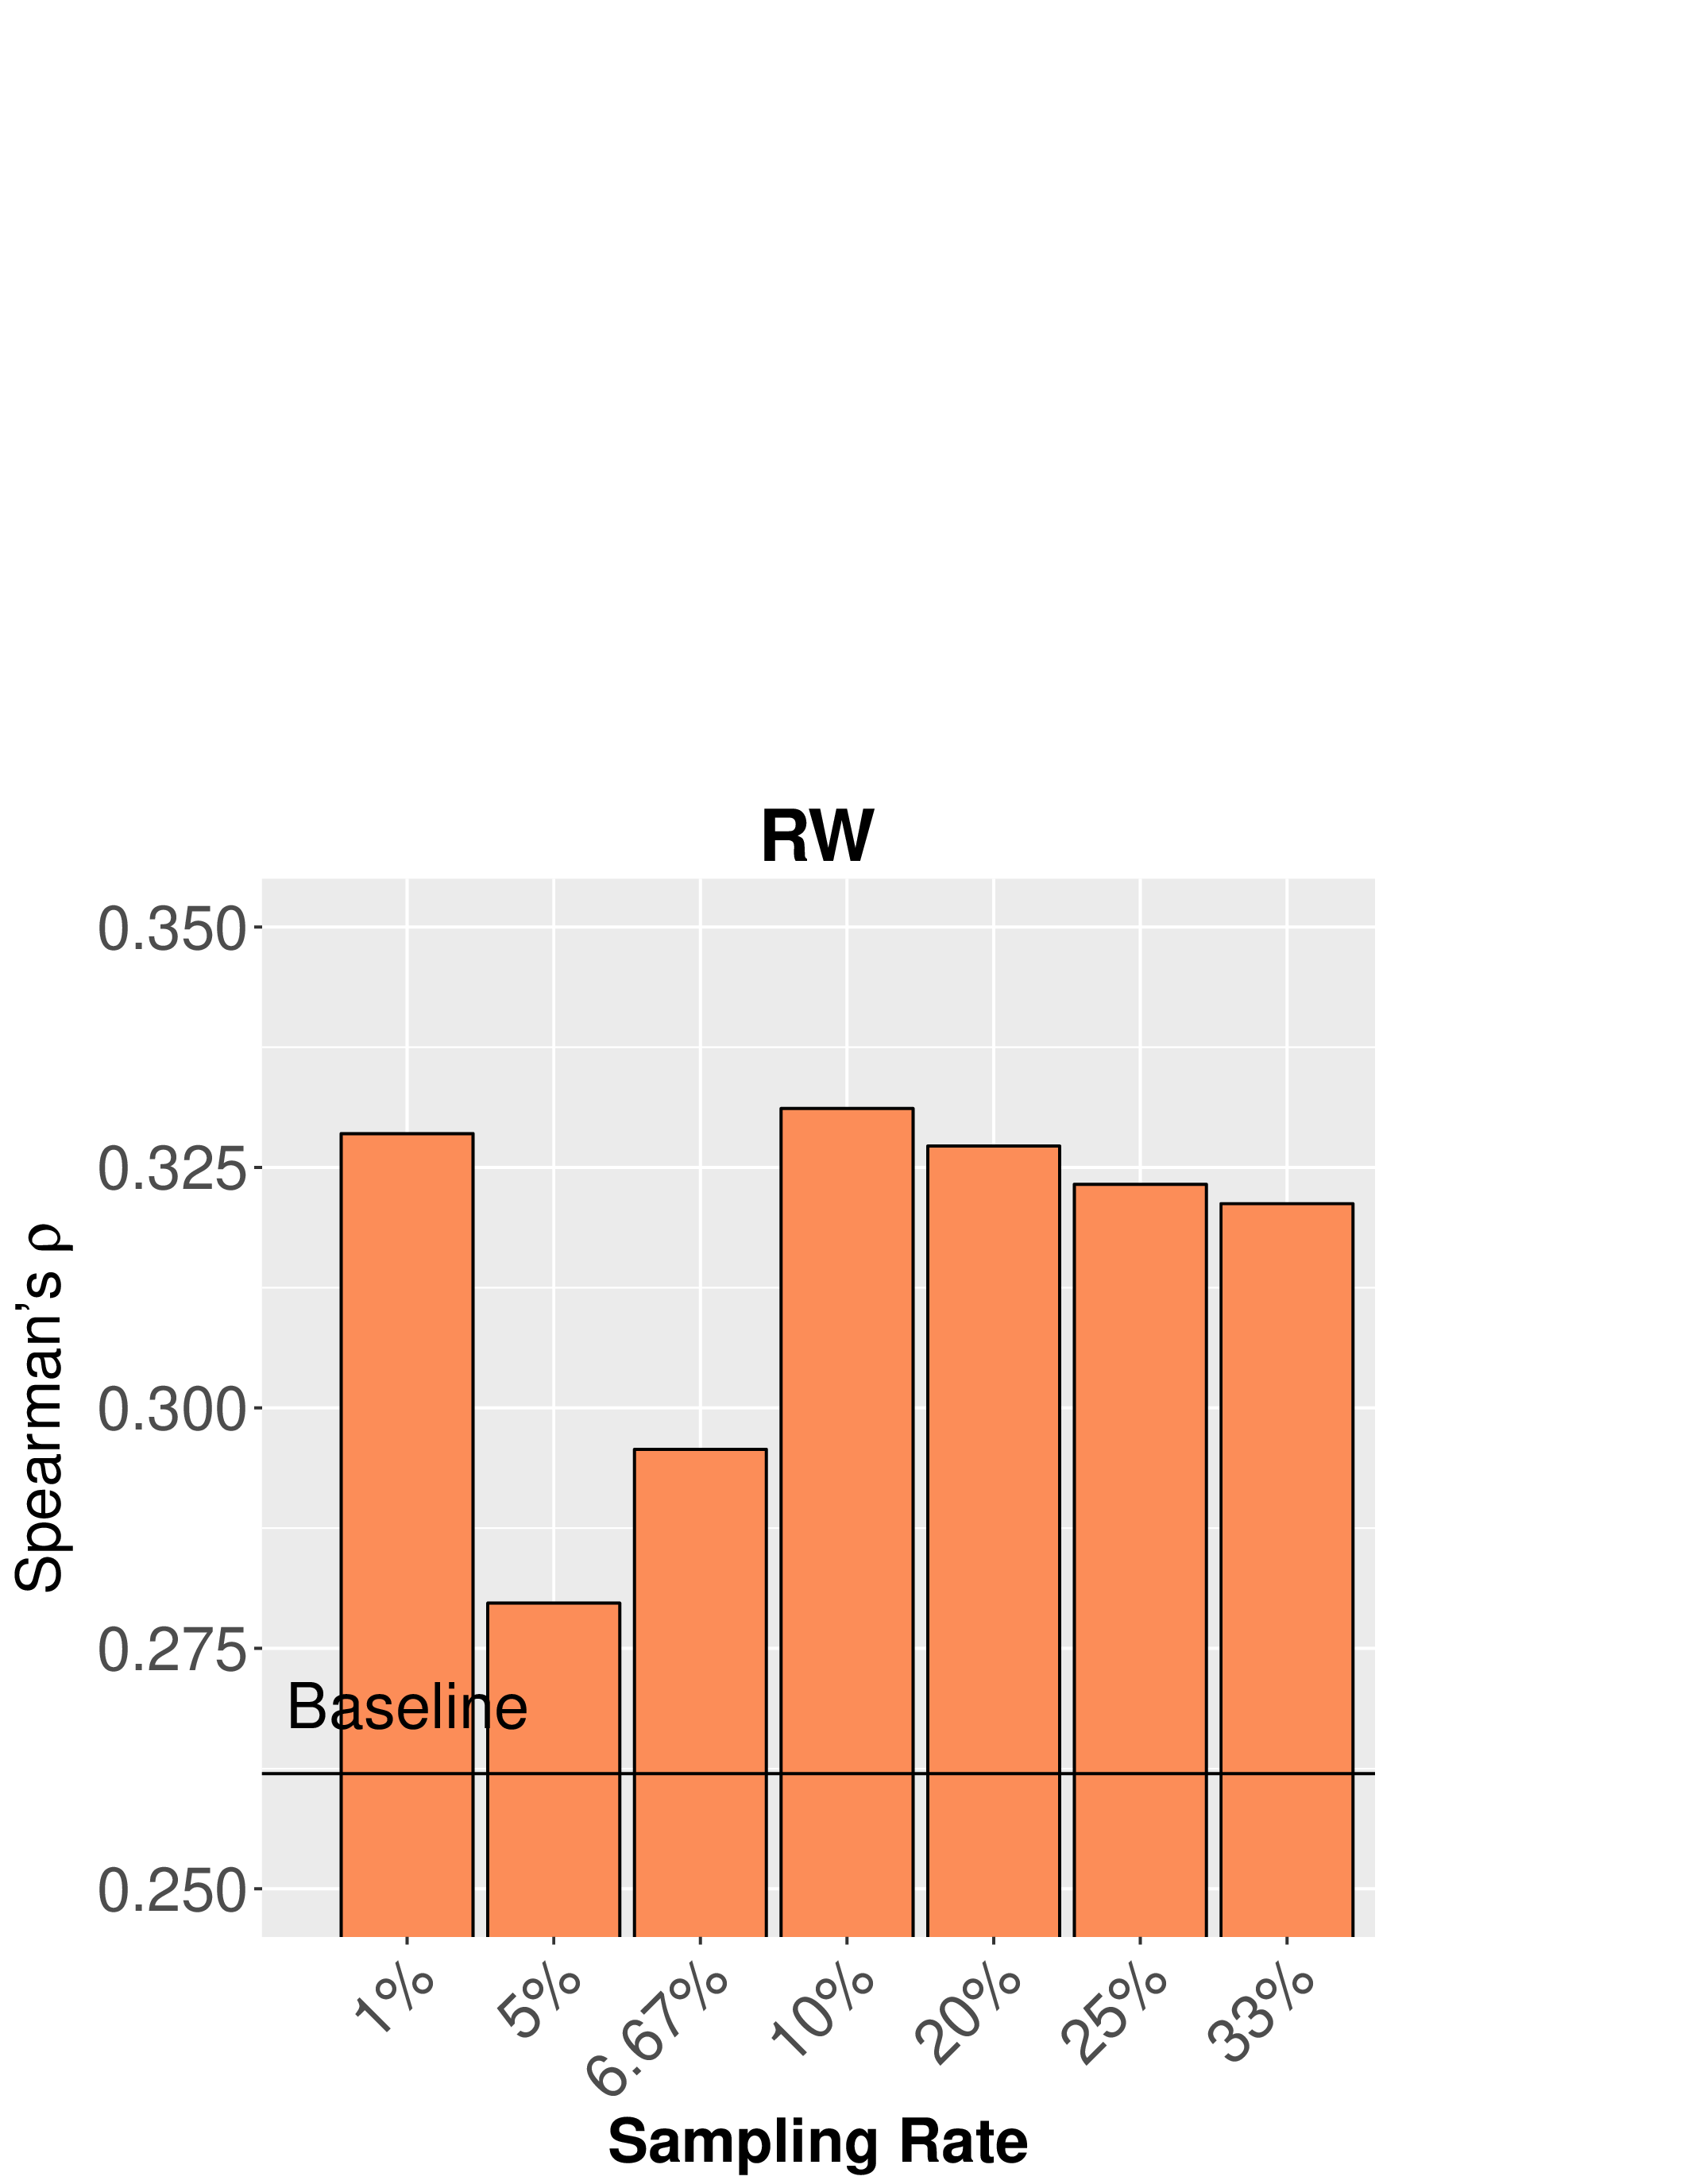}
	\end{subfigure}
    \begin{subfigure}{.24\linewidth}
   		\centering
   		\includegraphics[width=\linewidth]{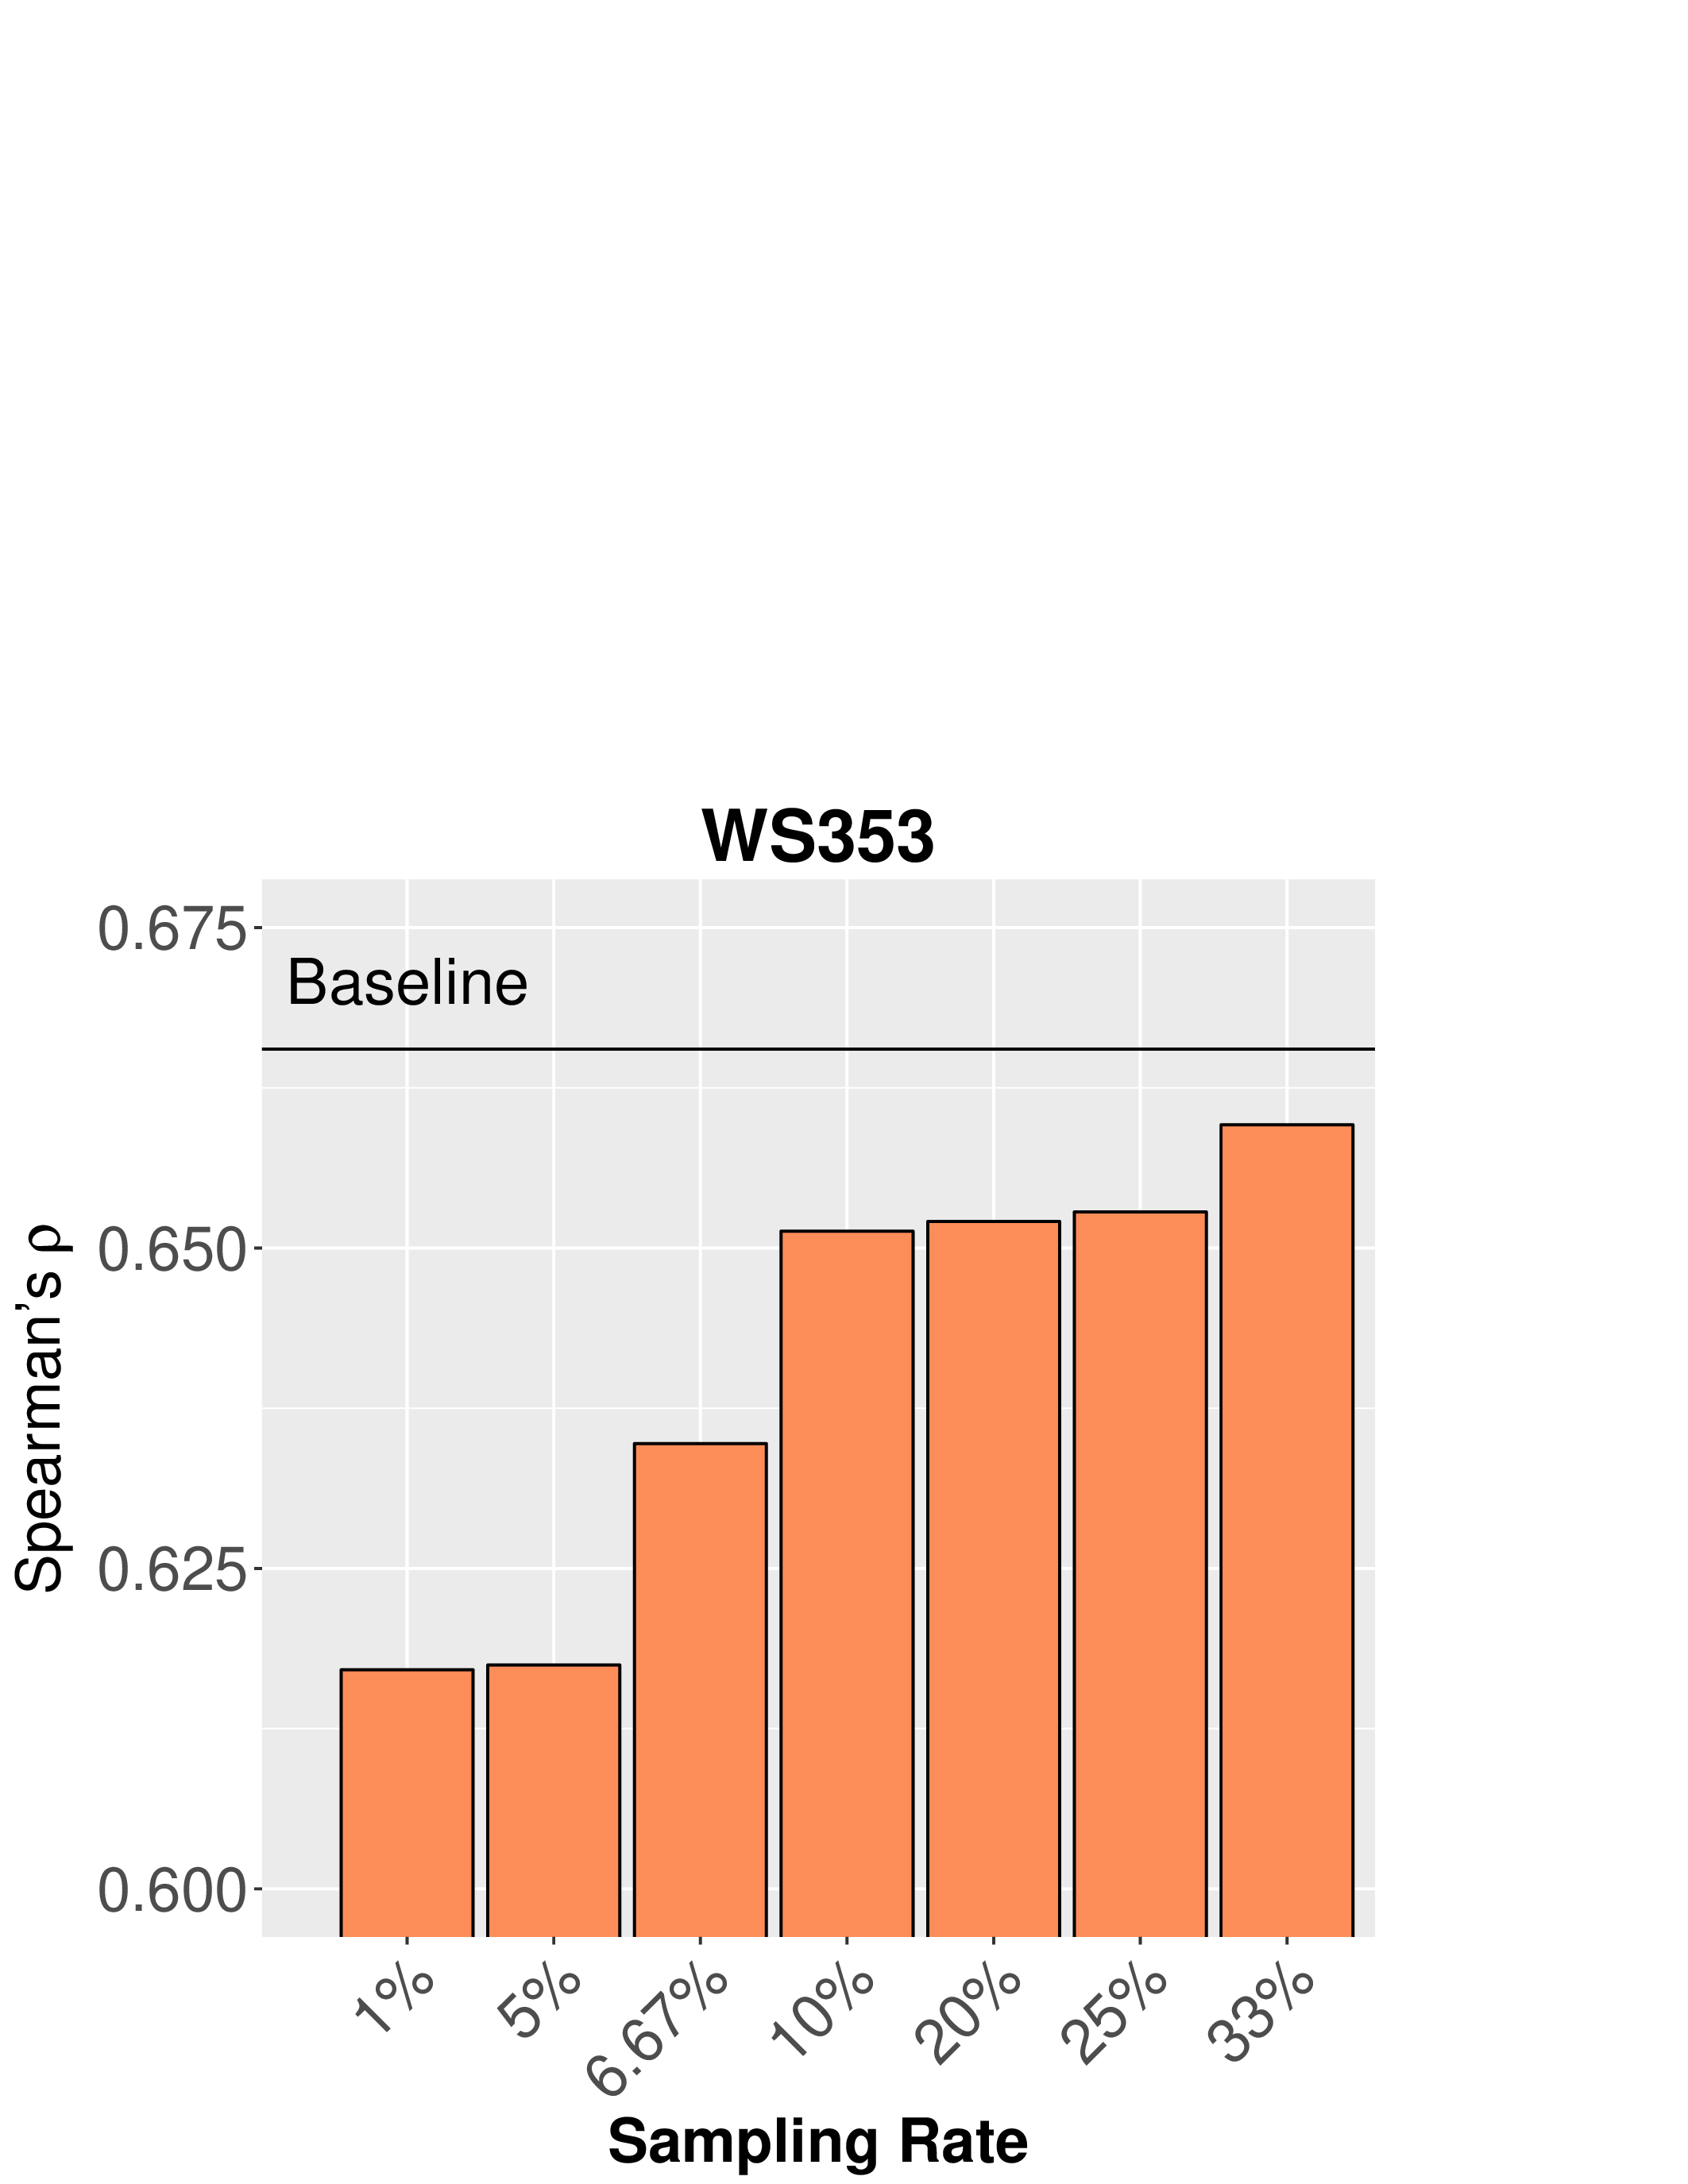}
    \end{subfigure}
    \begin{subfigure}{.24\linewidth}
    	\centering
  		\includegraphics[width=\linewidth]{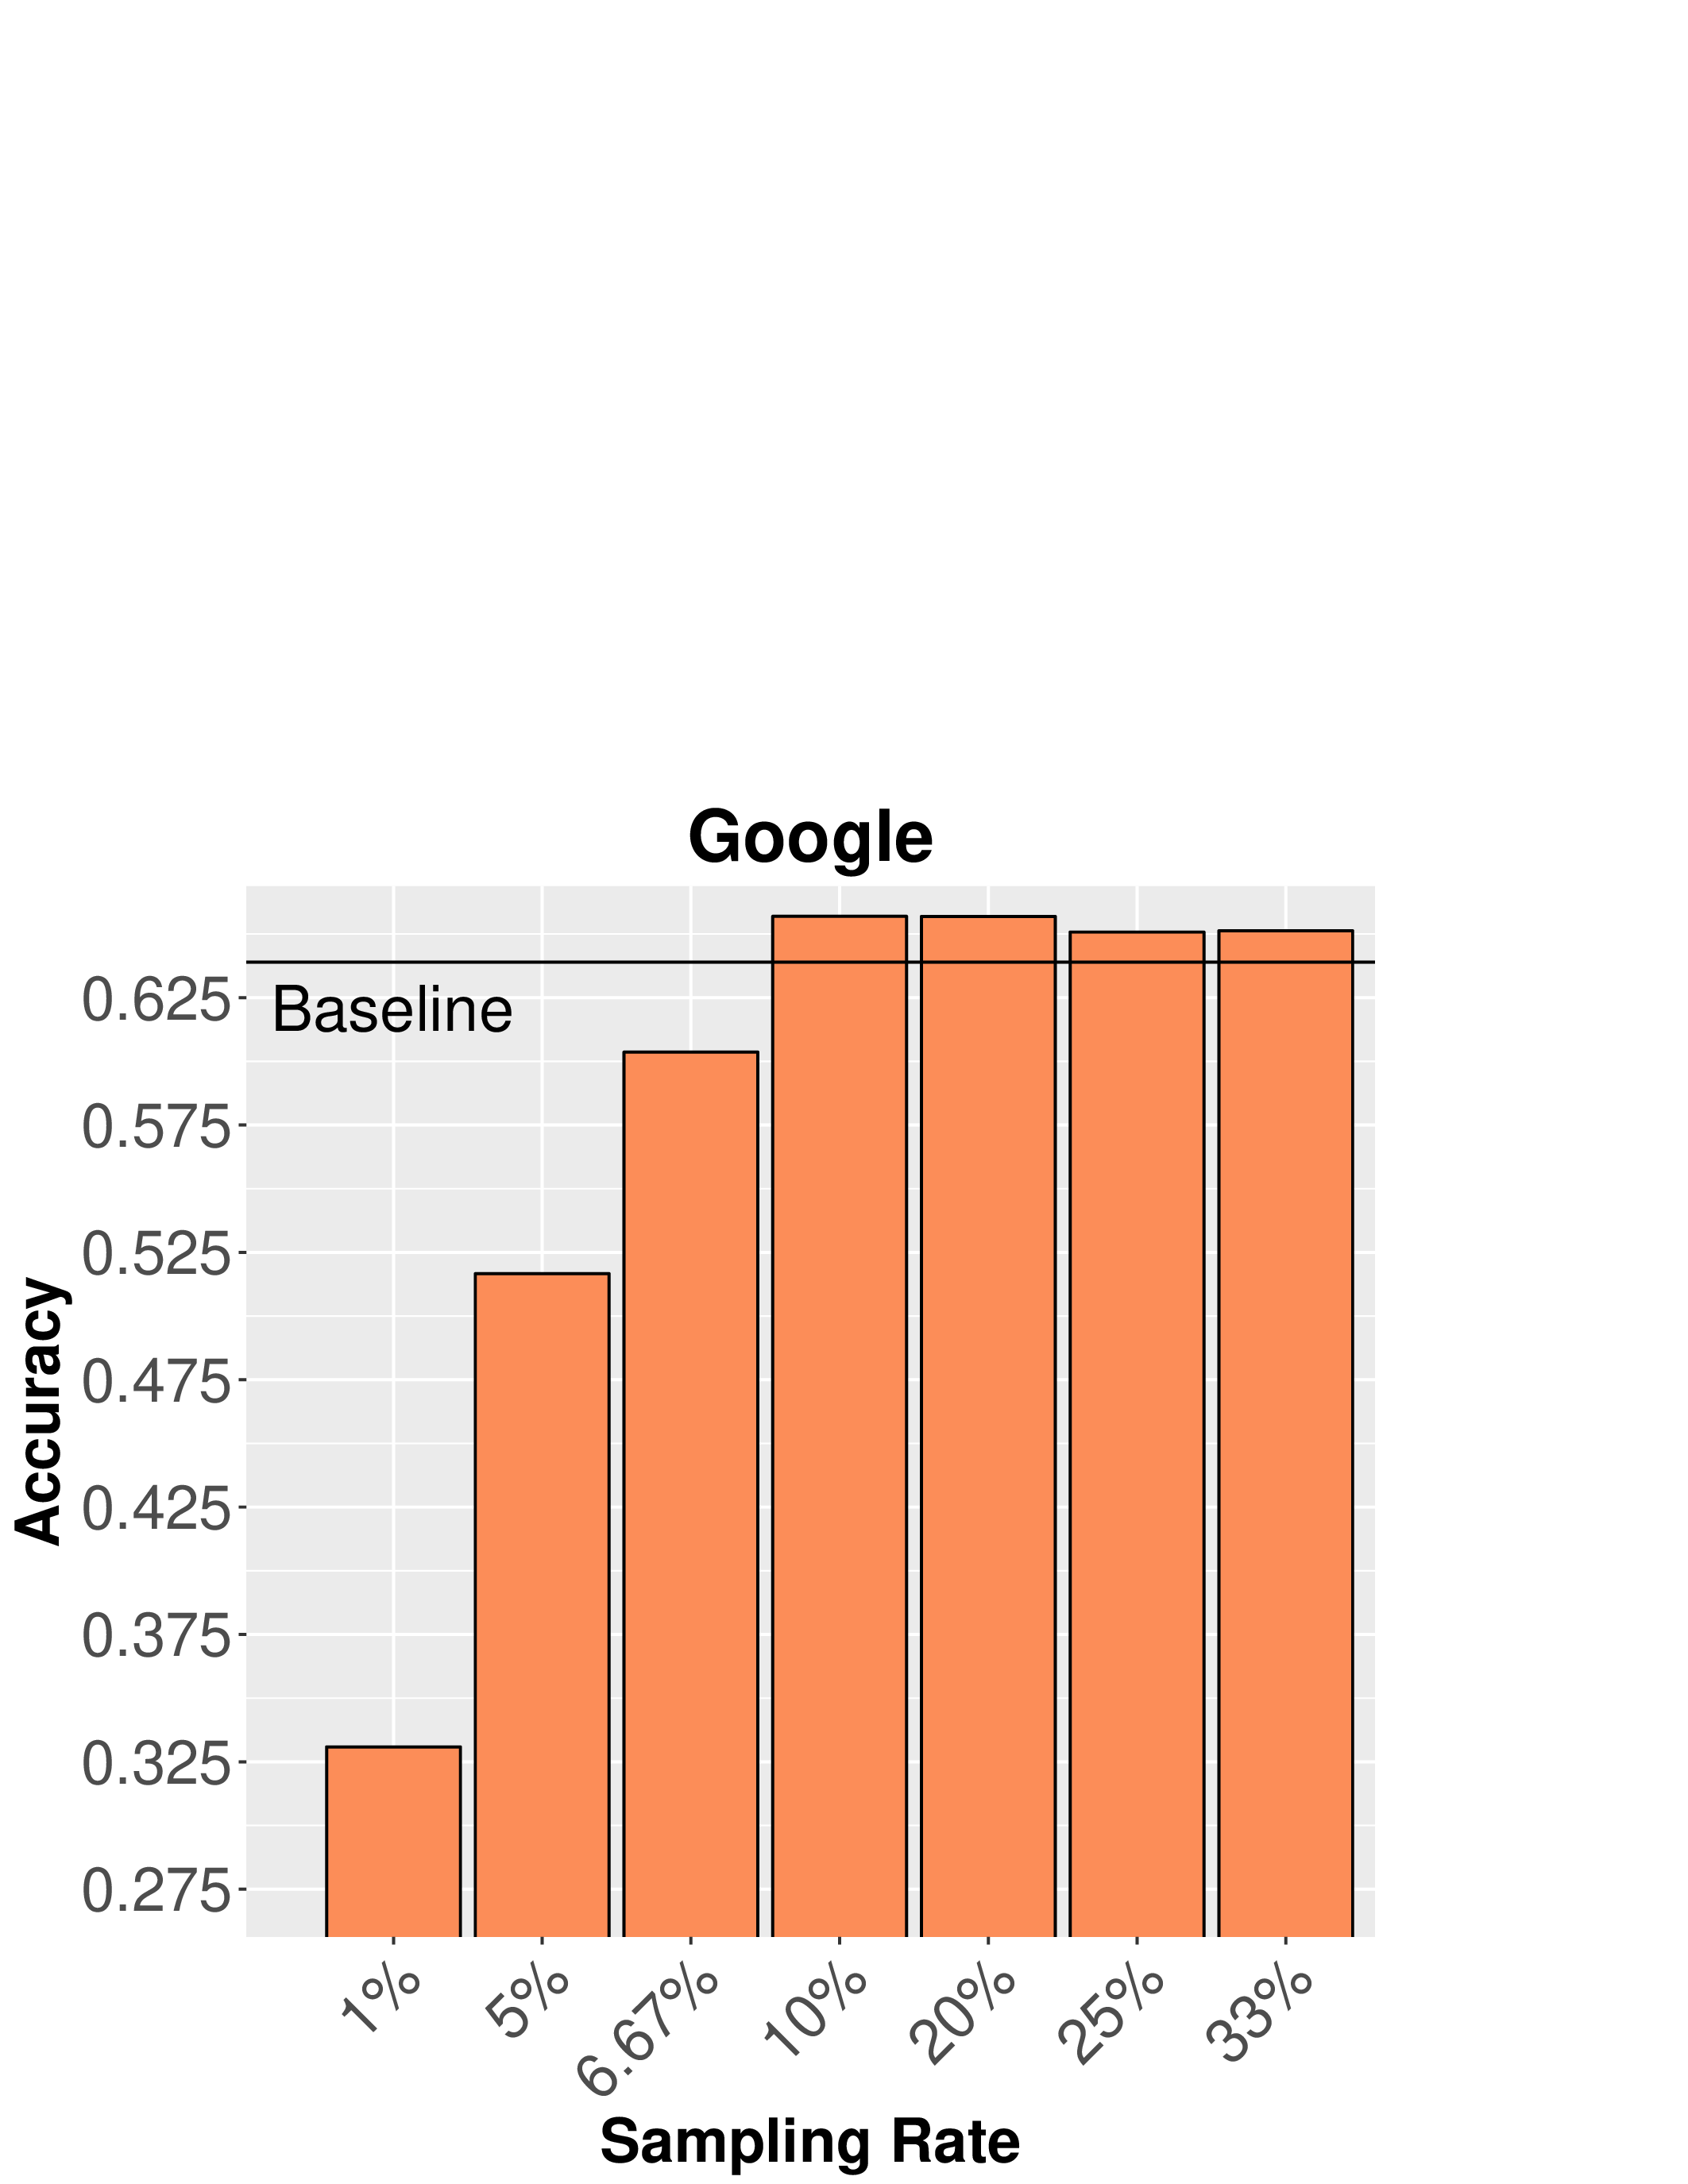}
    \end{subfigure}
    \begin{subfigure}{.24\linewidth}
	    \centering
  		\includegraphics[width=\linewidth]{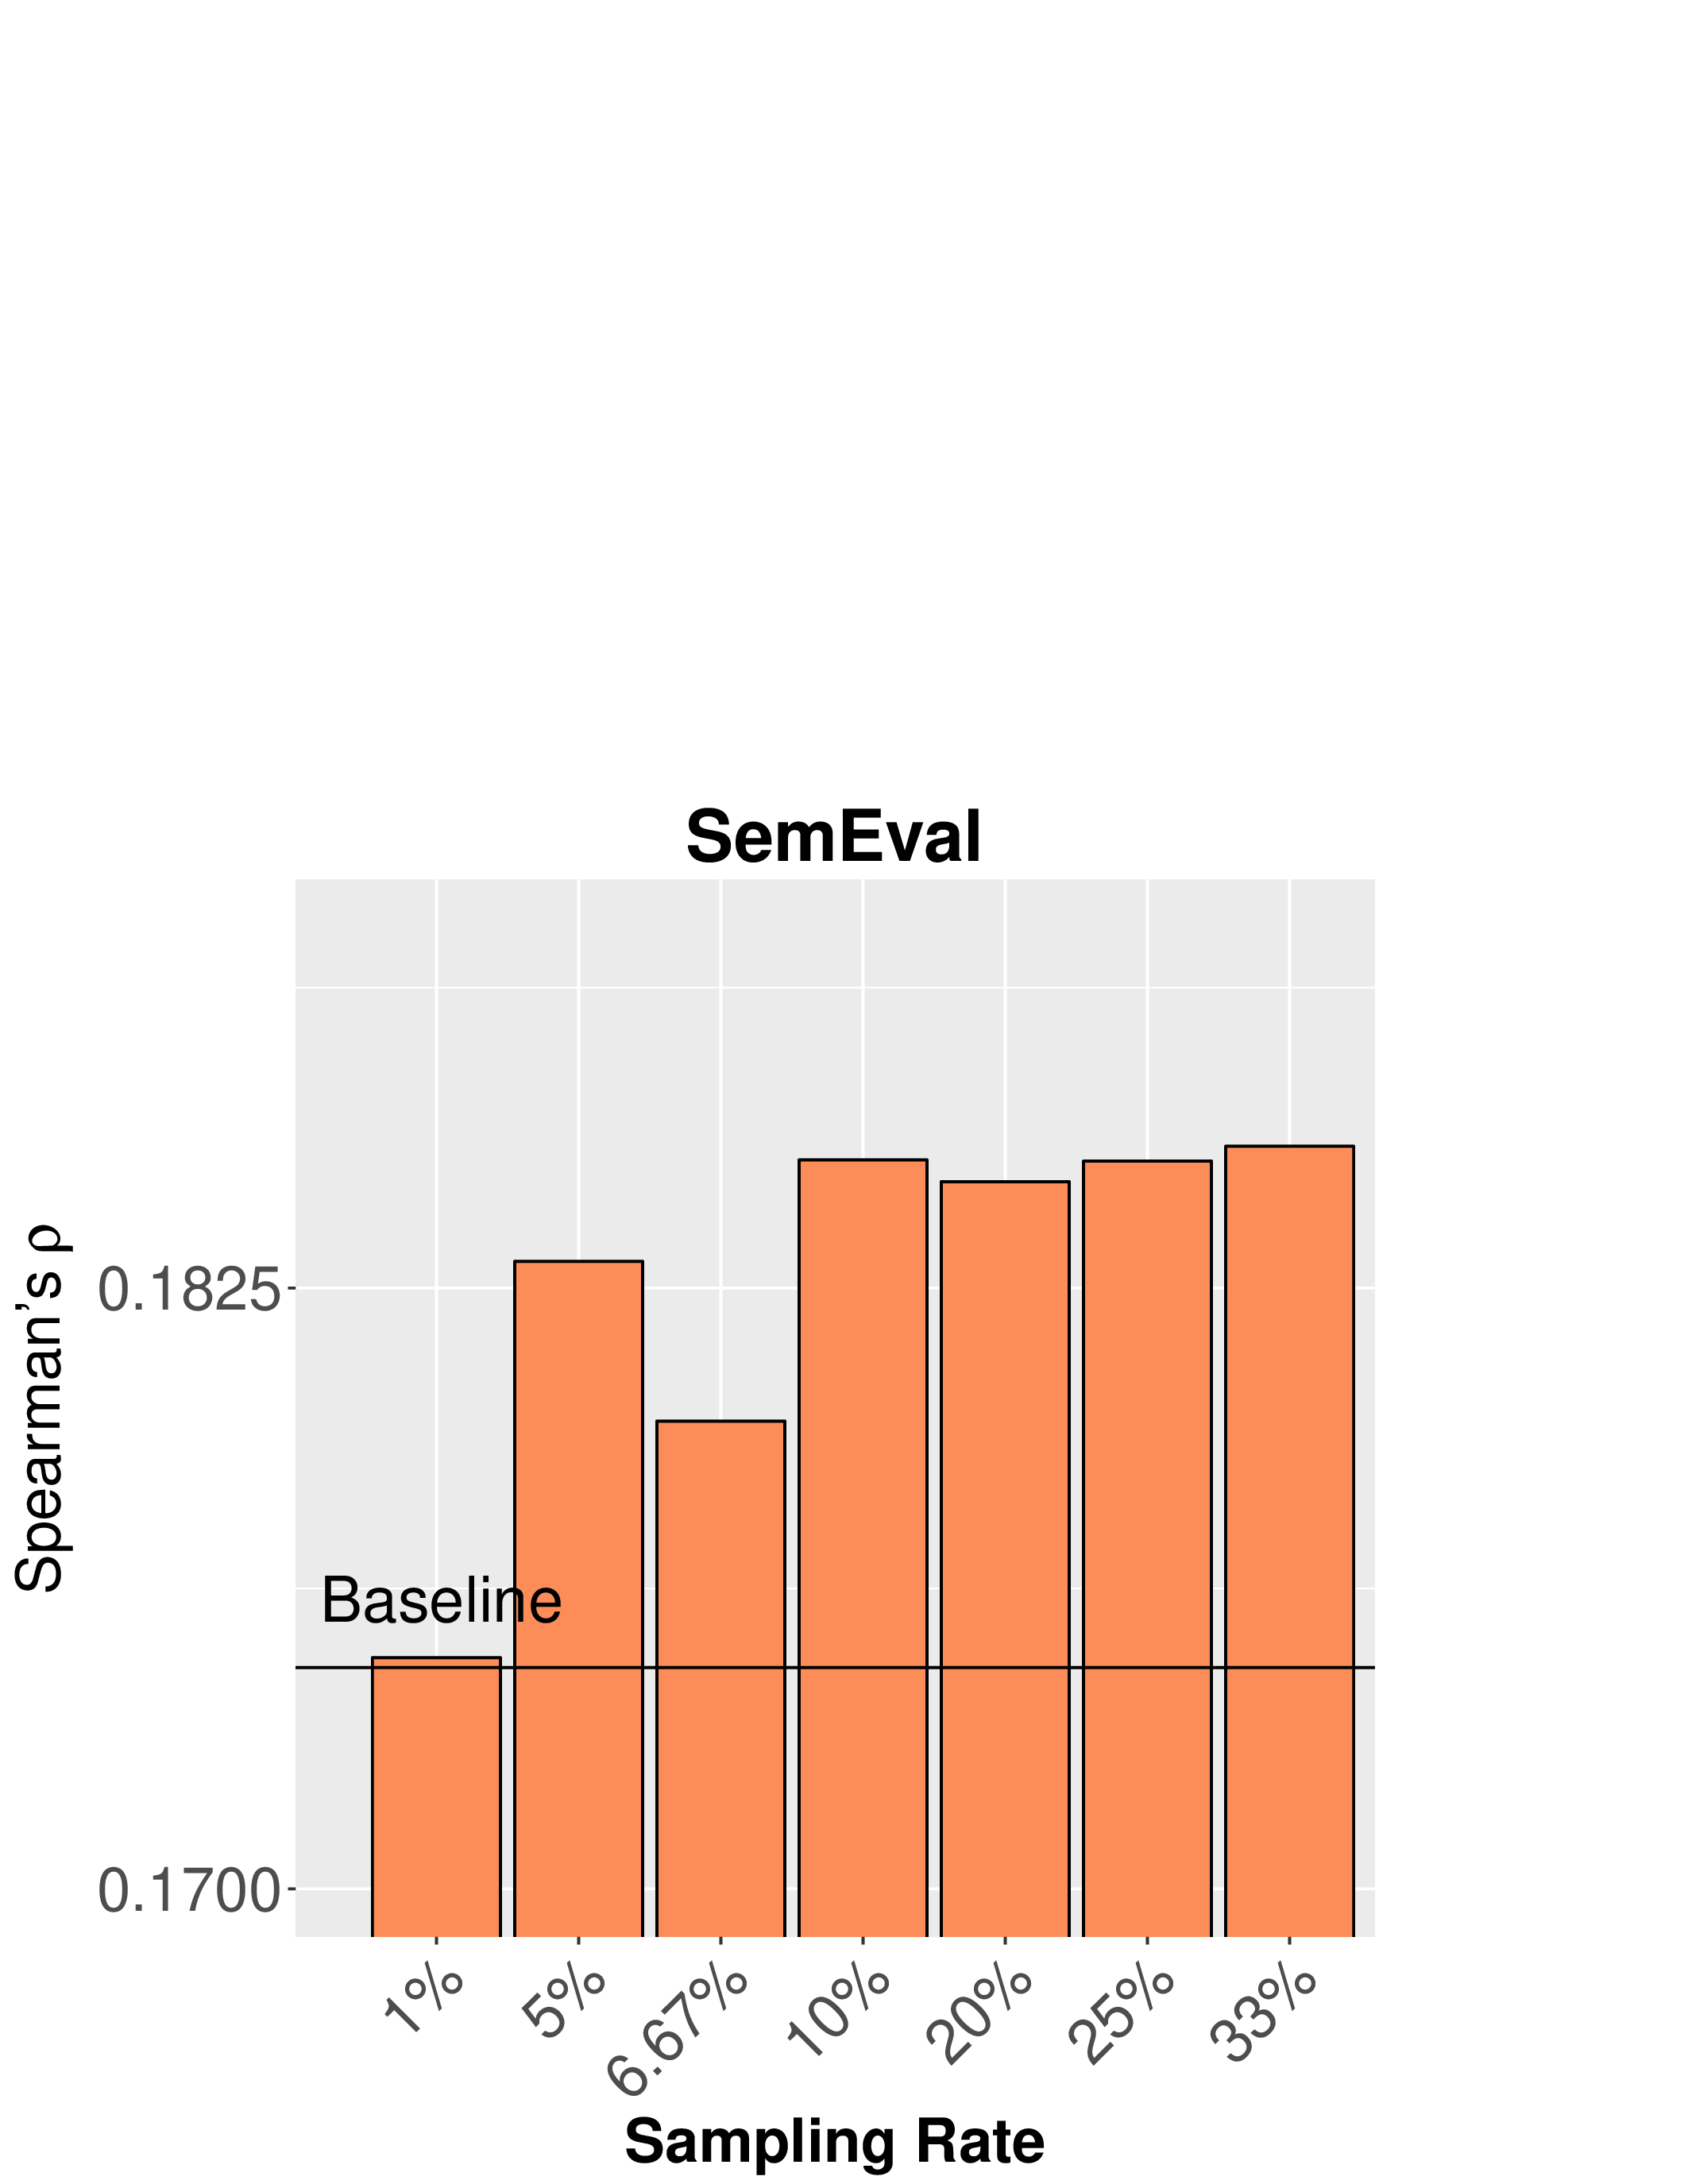}
    \end{subfigure}
    \caption{Comparison of different sampling rates on the Wikipedia data set. Merged using \problem. Sampled using \shuffle.}
	\label{fig:sampling-comparison}
\end{figure*}

\section{Effect of Sampling Rate and Sub-Model Counts}
\label{sec:sample-sizes-counts}
In this section, we first discuss results from an experiment where we vary the sampling rate $r$ while fixing the merging strategy (\problem) and sampling strategy (\shuffle). Then we discuss the results when varying only the number of sub-models being merged given a fixed sampling rate ($r$=10\%).

Figure~\ref{fig:sampling-comparison} illustrates the performance of our trained representations in various benchmarks for increasing sampling rates. We find two distinct trends here. 
For \ws, \google and \semeval, increased sampling rate (fewer sub-models) leads to better performance. This shows that increased parallelization does not always translate to good performance particularly in the analogy task which is considered to be a difficult task. Merging fewer sub-models that have encountered more training data is beneficial for these benchmarks. 

In the remaining 5/8 benchmarks, we find that lower sampling rates yield good results. 5-10\% sampling rate for our configuration gives the best results. With a lower sampling rate, training sub-models is considerably faster. Merging these models leads to good performance as well, with \baseline being bettered in all benchmarks except \men.  

Now we discuss the effect of merging a varying number of sub-models. Figure~\ref{fig:n-10-box} shows the relationship between count of merged sub-models and performance in each benchmark. We fix the $r$ as 10\% leading to a maximum of 10 sub-models. 

Immediately we can notice a steady increase in performance (in most benchmarks) as the number of sub-models merged increases. Benchmarks with more unique words benefit the most from merging more sub-models (see \ap vs \rw in Figure~\ref{fig:n-10-box}). When we select just a single model out of 10 (\#(sub-models) = 1), performance usually tends to be below the \baseline. This is especially true for \google and \battig where even the best model is worse than \baseline. 
Next we observe the plateauing of performance when merging more models. When utilizing a smaller sampling rate, this observation indicates that we can be more selective when merging. Instead of merging 100 sub-models produced when $r$=0.1\%, we can select a smaller number of sub-models on which to perform \problem. This is useful to speed up the overall training time since merging a large number of models using \problem is slow. This point is discussed in further detail in Section~\ref{sec:scaling}.

The performance also varies depending on the task at hand. We notice that for certain tasks/benchmarks merging new sub-models does not monotonically improve performance. For \rg, merging more than 3 sub-models is detrimental. For \semeval merging more than 5 decreases performance and similarly for \battig, 6 sub-models give best performance. 

These results show that merging more sub-models leads to improved performance over \baseline but for optimal performance in certain tasks we must carefully choose the number of sub-models to merge.
